# Supplementary material for: Nonlocal Effective Electromagnetic Wave Characteristics of Composite Media: Beyond the Quasistatic Regime
Source: arXiv:2007.00701 ancillary file (2021-03-16)
Supplement: Supplementary file 1 [file SupplementaryMaterial.pdf]

# Supplementary Material - Nonlocal Effective Electromagnetic Wave Characteristics of Composite Media: Beyond the Quasistatic Regime

Salvatore Torquato<sup>1,2,3,4,\*</sup> and Jaewuk Kim<sup>1</sup>

<sup>1</sup> Department of Physics, Princeton University, Princeton, New Jersey 08544, USA

<sup>2</sup> Department of Chemistry, Princeton University, Princeton, New Jersey 08544, USA

<sup>3</sup> Princeton Institute for the Science and Technology of Materials, Princeton University, Princeton, New Jersey 08544, USA

<sup>4</sup> Program in Applied and Computational Mathematics, Princeton University, Princeton, New Jersey 08544, USA

\* torquato@princeton.edu

## I. ORIGINAL LOCAL STRONG-CONTRAST EXPANSIONS

Here we state the original local strong-contrast expansions obtained by Rechtsman and Torquato [1] and then discuss approximations extracted from them. The expansions are valid only in the quasistatic regime because they are derived from a homogenized constitutive relation that is local in space. The problem setup is the same as the one discussed in Sec. IV in the main text. The original Rechtsman-Torquato quasistatic strong-contrast expansion for the effective dielectric constant tensor  $\varepsilon_e$  is given by

$$(\phi_p \beta_{pq})^2 \left[ \frac{\varepsilon_e(k_q) - \varepsilon_q \mathbf{I}}{\varepsilon_e(k_q) + (d-1)\varepsilon_q \mathbf{I}} \right]^{-1} = \phi_p \beta_{pq} \mathbf{I} - \sum_{n=2}^{\infty} \mathbf{A}_n^{(p)}(k_q) \beta_{pq}^n, \quad (\text{S1})$$

where

$$\beta_{pq} \equiv \frac{\varepsilon_p - \varepsilon_q}{\varepsilon_p + (d-1)\varepsilon_q} \quad (\text{S2})$$

is the dielectric *polarizability*, and the  $n$ -point local parameters  $\mathbf{A}_n^{(p)}(k_q)$  are defined as

$$\mathbf{A}_2^{(p)}(k_q) = d\varepsilon_q \int_{\epsilon} \mathbf{H}^{(q)}(\mathbf{r}_1) \chi_V(\mathbf{r}_1) d\mathbf{r}_1, \quad (\text{S3})$$

$$\begin{aligned} \mathbf{A}_n^{(p)}(k_q) = & d\varepsilon_q \left( \frac{-d\varepsilon_q}{\phi_p} \right)^{n-2} \int_{\epsilon} \mathbf{H}^{(q)}(\mathbf{x}_1 - \mathbf{x}_2) \cdots \mathbf{H}^{(q)}(\mathbf{x}_{n-1} - \mathbf{x}_n) \\ & \times \Delta_n^{(p)}(\mathbf{x}_1, \dots, \mathbf{x}_n) d\mathbf{x}_2 \cdots d\mathbf{x}_n, \quad n \geq 3, \end{aligned} \quad (\text{S4})$$

where  $\int_{\epsilon} d\mathbf{r} = \lim_{\epsilon \rightarrow 0^+} \int_{|\mathbf{r}| > \epsilon} d\mathbf{r}$  for a spherical exclusion region, the explicit formula of the second-rank tensor field  $\mathbf{H}^{(q)}(\mathbf{r})$  is given in Eq. (S32), and  $\Delta_n^{(p)}(\mathbf{x}_1, \dots, \mathbf{x}_n)$  is a position-dependent determinant involving up to the  $n$ -point correlation function associated with the polarized phase  $p$  of composites, given in Eq. (53) in the main text.

### Remarks:

1. The effective dielectric constant tensor  $\varepsilon_e$  depends on the wavenumber  $k_q$  of the applied electric field in the reference phase. Importantly, while the resulting tensor  $\varepsilon_e$  can be anisotropic, it is expected to be independent of the propagation direction of the applied field.
2. The  $n$ -point parameters  $\mathbf{A}_n^{(p)}(k_q)$  given in Eqs. (S3) and (S4) are different from those for the nonlocal strong-contrast expansions beyond the quasistatic regime; see Sec. II.
3. The homogenized relation for the original strong-contrast expansion is local in space:

$$\langle \mathbf{P} \rangle(\mathbf{x}) = \mathbf{L}_e^{(q)}(\mathbf{k} = \mathbf{0}) \cdot \langle \mathbf{F} \rangle(\mathbf{x}), \quad (\text{S5})$$

where ensemble averages  $\langle \mathbf{P} \rangle(\mathbf{x})$  and  $\langle \mathbf{F} \rangle(\mathbf{x})$  are constants of position. The reader is referred to as Eq. (S48) for the nonlocal counterpart that is derived in the present work.

4. The second-rank tensor field  $\mathbf{H}^{(q)}(\mathbf{r})$  given in Eq. (S32) is related to  $\mathbf{t}^{(p)}(\mathbf{r})$  given in Eq. (19) in Ref. [1] as follows:

$$\mathbf{t}^{(p)}(\mathbf{r}) = \Omega_d \varepsilon_q \mathbf{H}^{(q)}(\mathbf{r}),$$

where  $\Omega_d$  is the surface area of a  $d$ -dimensional unit sphere.

### A. Truncated Approximations

For the reasons that we discussed in Sec. III in the main text, truncation of expansions (S1) at the  $n$ -point level gives an accurate approximation of  $\varepsilon_e$  for two-phase composites. We present the two- and three-point approximations of the original strong-contrast expansions, derived in Ref. [1], for the macroscopically isotropic media. In this case, the effective dielectric constant tensor  $\varepsilon_e(k_q)$  can be reduced to a scalar quantity  $\varepsilon_e(k_q)$  by taking the trace, i.e.,  $\varepsilon_e(k_q) = \text{Tr}[\varepsilon_e(k_q)]/d$ .

The two-point approximation is obtained by setting  $\mathbf{A}_n^{(p)} = \mathbf{0}$  for  $n \geq 3$  in Eq. (S1), taking trace of its both sides, and solving them in  $\varepsilon_e(k_q)$ :

$$\begin{aligned} \frac{\varepsilon_e(k_q)}{\varepsilon_q} &= 1 + \frac{d\beta_{pq}\phi_p^2}{\phi_p(1 - \beta_{pq}\phi_p) - \beta_{pq}A_2^{(p)}(k_q)} \\ &= 1 + \frac{d\beta_{pq}\phi_p^2}{\phi_p(1 - \beta_{pq}\phi_p) + (d-1)\pi/[2^{d/2}\Gamma(d/2)]\beta_{pq}\mathcal{F}(k_q)}, \end{aligned} \quad (\text{S6})$$

where  $\Gamma(x)$  is the Gamma function,  $\beta_{pq}$  is defined in Eq. (S2), and  $A_n^{(p)} \equiv \text{Tr}[\mathbf{A}_n^{(p)}]/d$  for  $n = 2, \dots$ . Here the local attenuation function  $\mathcal{F}(Q)$  is defined as

$$\mathcal{F}(Q) \equiv -\frac{2^{d/2}\Gamma(d/2)}{\pi}Q^2 \int_{\epsilon} \frac{i}{4} \left( \frac{Q}{2\pi r} \right)^{d/2-1} \mathcal{H}_{d/2-1}^{(1)}(Qr) \chi_v(r) \, \text{d}r \quad (\text{S7})$$

$$= -\frac{\Gamma(d/2)}{2^{d/2}\pi^{d+1}}Q^2 \int \frac{\tilde{\chi}_v(\mathbf{q})}{|\mathbf{q}|^2 - Q^2} \, \text{d}\mathbf{q}, \quad (\text{S8})$$

where  $\mathcal{H}_\nu^{(1)}(x)$  is the Hankel function of the first kind of order  $\nu$ , and Eq. (S8) is obtained by applying the Parseval theorem to Eq. (S7). Importantly, we note that the integrand in Eq. (S8) depends on the shape of the exclusion-region; see Sec. II A for details.

Analogously, the three-point approximation is obtained from Eq. (S1) as follows:

$$\frac{\varepsilon_e(k_q)}{\varepsilon_q} = 1 + \frac{d\beta_{pq}\phi_p^2}{\phi_p(1 - \beta_{pq}\phi_p) - \beta_{pq}A_2^{(p)}(k_q) - \beta_{pq}^2A_3^{(p)}(k_q)}, \quad (\text{S9})$$

where the three-point local parameter is given as

$$A_3^{(p)}(k_q) \equiv -\frac{(d\varepsilon_q)^2}{\phi_p} \int_{\epsilon} \text{d}\mathbf{x}_2 \, \text{d}\mathbf{x}_3 \, \frac{1}{d} \text{Tr}[\mathbf{H}^{(q)}(\mathbf{x}_1 - \mathbf{x}_2) \cdot \mathbf{H}^{(q)}(\mathbf{x}_2 - \mathbf{x}_3)] \Delta_3^{(p)}(\mathbf{x}_1, \mathbf{x}_2, \mathbf{x}_3) \quad (\text{S10})$$

$$\begin{aligned} &= -\frac{1}{\phi_p(2\pi)^{2d}} \int \text{d}\mathbf{q}_1 \, \text{d}\mathbf{q}_2 \, \frac{1}{q_1^2 - k_q^2} \frac{1}{q_2^2 - k_q^2} \left\{ (d-1)^2 k_q^4 + q_1^2 q_2^2 [d(\hat{\mathbf{q}}_1 \cdot \hat{\mathbf{q}}_2)^2 - 1] \right\} \\ &\quad \times \tilde{\Delta}_3^{(p)}(\mathbf{q}_1, \mathbf{q}_2), \end{aligned} \quad (\text{S11})$$

where, due to the statistical homogeneity,

$$\tilde{\Delta}_3^{(p)}(\mathbf{q}_1, \mathbf{q}_2) = \int \text{d}\mathbf{r}_1 \, \text{d}\mathbf{r}_2 \, e^{-i\mathbf{q}_1 \cdot \mathbf{r}_1} e^{-i\mathbf{q}_2 \cdot \mathbf{r}_2} [S_2^{(p)}(\mathbf{r}_1) S_2^{(p)}(\mathbf{r}_2) - \phi_p S_3^{(p)}(\mathbf{r}_1, \mathbf{r}_2)].$$

### B. Properties of the Local Attenuation Function $\mathcal{F}(Q)$

Assuming both  $\varepsilon_1$  and  $\varepsilon_2$  are real-valued, the imaginary part of the local attenuation function  $\mathcal{F}(Q)$  determines the attenuation characteristics of a composite predicted by the two-point approximation (S6). In this subsection, we investigate some generic and microstructure-dependent properties of  $\mathcal{F}(Q)$ . We compare  $\mathcal{F}(Q)$  to its nonlocal counterpart defined in Eq. (S89) in Sec. IV.

For statistically isotropic media, the real and imaginary parts of local attenuation function, defined in Eq. (S7),

can be simplified as

$$\text{Im}[\mathcal{F}(Q)] = - \lim_{\epsilon \rightarrow 0^+} \int_{\epsilon}^{\infty} dr Q \chi_{\nu}(r) (Qr)^{d/2} J_{d/2-1}(Qr) \quad (\text{S12})$$

$$= - \frac{Q^d}{(2\pi)^{d/2}} \tilde{\chi}_{\nu}(Q), \quad (\text{S13})$$

$$\text{Re}[\mathcal{F}(Q)] = \lim_{\epsilon \rightarrow 0^+} \int_{\epsilon}^{\infty} dr Q \chi_{\nu}(r) (Qr)^{d/2} Y_{d/2-1}(Qr) \quad (\text{S14})$$

$$= - \frac{2Q^2}{\pi} \text{p.v.} \int_0^{\infty} dq \frac{1}{q(Q^2 - q^2)} \text{Im}[\mathcal{F}(q)], \quad (\text{S15})$$

where  $J_{\nu}(x)$  [ $Y_{\nu}(x)$ ] is the Bessel function of the first kind [the second kind] of order  $\nu$ , and p.v. stands for the Cauchy principal value of an integral. For a finite  $Q$ , the limits of integrals in Eqs. (S12) and (S14) can be simplified to  $\int_0^{\infty} dr$  because the integrands do not possess a singularity at the origin. Equation (S15) is obtained from Eqs. (S12) and (S14) by utilizing the following identity

$$Y_{\nu-1}(Qr) = \text{p.v.} \int_0^{\infty} dq \frac{q^{\nu}}{Q^2 - q^2} J_{\nu-1}(qr), \quad (\text{S16})$$

for positive real numbers  $Q$ ,  $r$ , and  $\nu$ .

Using the formulas above, we investigate the asymptotic behaviors of  $\mathcal{F}(Q)$  in both quasistatic (small- $Q$ ) and large- $Q$  regimes. For the imaginary part  $\text{Im}[\mathcal{F}(Q)]$ , those expressions can be easily obtained from Eq. (S13) and the asymptotic behaviors of the spectral density  $\tilde{\chi}_{\nu}(Q)$ . For either nonhyperuniform or hyperuniform isotropic media, the spectral density has the following power-law scalings:

$$\tilde{\chi}_{\nu}(Q) \sim \begin{cases} Q^{\alpha}, & \text{in the quasistatic regime,} \\ Q^{-(d+1)}, & \text{in the large-}Q \text{ regime,} \end{cases} \quad (\text{S17})$$

where the exponent  $\alpha$  lies in the interval  $(0, \infty)$  for hyperuniform systems, and  $\alpha = 0$  for nonhyperuniform systems. Combining Eqs. (S13) and (S17) immediately gives

$$\text{Im}[\mathcal{F}(Q)] \sim \begin{cases} Q^{d+\alpha}, & \text{in the quasistatic regime,} \\ Q^{-1}, & \text{in the large-}Q \text{ regime.} \end{cases} \quad (\text{S18})$$

By contrast, for both hyperuniform and nonhyperuniform systems, the real part exhibits common asymptotic behaviors

$$\text{Re}[\mathcal{F}(Q)] \sim Q^2, \quad \text{in the quasistatic regime,} \quad (\text{S19})$$

$$\text{Re}[\mathcal{F}(Q)] \rightarrow \frac{2^{d/2} \Gamma(d/2)}{\pi} \phi_p (1 - \phi_p), \quad \text{in the large-}Q \text{ regime.} \quad (\text{S20})$$

Expression (S19) is obtained from Eq. (S14) by using the Taylor expansion of  $Y_{\nu}(x)$  around the origin:

$$\text{Re}[\mathcal{F}(Q)] \sim Q^2 \int_0^{\infty} dr r \chi_{\nu}(r) \sim Q^2. \quad (\text{S21})$$

In order to obtain Eq. (S20), we use Eqs. (S13) and (S15) to write

$$\begin{aligned} \text{Re}[\mathcal{F}(Q)] &= \frac{2Q^2}{\pi} \frac{1}{(2\pi)^{d/2}} \text{p.v.} \int_0^{\infty} dq \frac{q^{d-1}}{Q^2 - q^2} \tilde{\chi}_{\nu}(q) \\ &= \frac{2}{\pi} \frac{1}{(2\pi)^{d/2}} \text{p.v.} \int_0^{\infty} dq \frac{q^{d-1}}{1 - (q/Q)^2} \tilde{\chi}_{\nu}(q). \end{aligned}$$

Since  $q^{d-1} \tilde{\chi}_{\nu}(q)$  vanishes like  $1/q^2$  for large  $q$ , the singularity contribution in this integral can be neglected in the large- $Q$  limit

$$\lim_{Q \rightarrow \infty} \text{Re}[\mathcal{F}(Q)] \approx \frac{2}{\pi} \frac{1}{(2\pi)^{d/2}} \int_0^{\infty} dq q^{d-1} \tilde{\chi}_{\nu}(q) = \frac{2^{d/2} \Gamma(d/2)}{\pi} \phi_p (1 - \phi_p),$$

where we note that the integral above is related to the inverse Fourier transform of  $\tilde{\chi}_v(q)$  at  $r = 0$ , i.e.,

$$\frac{1}{(2\pi)^d} \int_0^\infty dq \frac{2\pi^{d/2}}{\Gamma(d/2)} q^{d-1} \tilde{\chi}_v(q) = \chi_v(0) = \phi_p(1 - \phi_p).$$

We present the local attenuation function  $\mathcal{F}(Q)$  for the four models of three-dimensional disordered composite media, discussed in the main text; see Fig. S1. In the inset of the lower panel of this figure, one can see how the power-law scalings vary with models in the quasistatic regime.

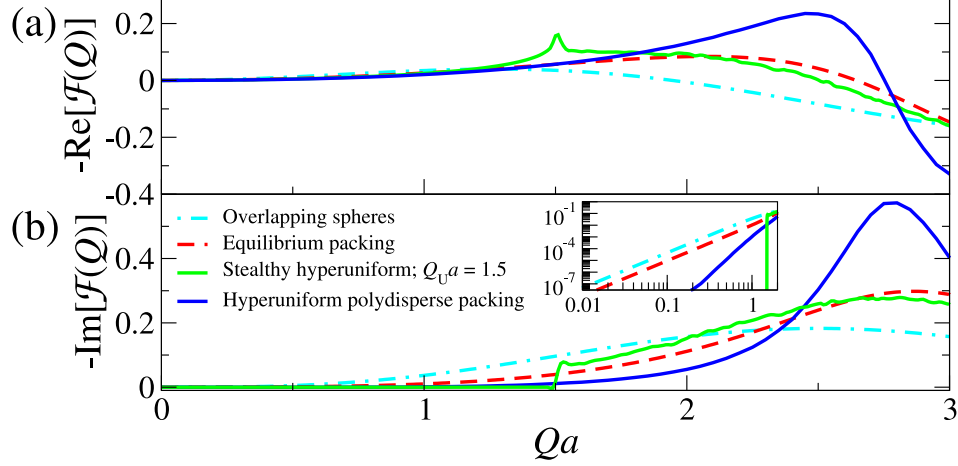

FIG. S1. Evaluation of the negative values of (a) the real and (b) negative imaginary parts of the local attenuation function  $\mathcal{F}(Q)$ , defined in Eq. (S7), as a function of dimensionless wavenumber  $Qa$  for the four models of three-dimensional disordered particulate media. Each model has the same volume fraction for the dispersed phase  $\phi_2 = 0.25$ . The inset in (b) is the log-log plot of the larger panel. The first three models consist of spheres of radius  $a$ . For class I hyperuniform packings via tessellation-based procedure,  $a$  is the mean sphere radius, i.e.,  $\phi_2 = \rho v_1(a)$ , where  $\rho$  is number density of particle centers, and  $v_1(a)$  is the volume of a  $d$  dimensional sphere of radius  $a$ .

## II. DERIVATIONS OF NONLOCAL STRONG-CONTRAST EXPANSION

Here we present a detailed derivation of the nonlocal strong-contrast expansion presented in the main text. Aforementioned, we consider a macroscopically large ellipsoidal two-phase composite specimen in  $\mathbb{R}^d$  embedded inside an infinitely large reference phase of dielectric constant tensor  $\epsilon_I$ . We assume that the microstructure is perfectly general, and the inhomogeneity length scales  $\ell$  are much smaller than the size of specimen  $L$ , i.e.,  $\ell \ll L$ . The shape of this specimen is purposely chosen to be non-spherical since any rigorously correct expression for the effective stiffness tensor must ultimately be independent of the shape of the composite specimen in the infinite-volume limit. The local dielectric constant tensor  $\epsilon(\mathbf{x})$  of a two-phase composite is written as

$$\epsilon(\mathbf{x}) \equiv \epsilon_1 \mathcal{I}^{(1)}(\mathbf{x}) + \epsilon_2 \mathcal{I}^{(2)}(\mathbf{x}), \quad (\text{S22})$$

where  $\epsilon_i$  is the dielectric constant tensor of phase  $i = 1, 2$ , and  $\mathcal{I}^{(i)}(\mathbf{x})$  is the indicator of phase  $i$  (see Sec. II in the main text). It is assumed that the incident electric wave  $\mathbf{E}_0(\mathbf{x})$  is a plane wave of an angular frequency  $\omega$  and wavevector  $\mathbf{k}_I(\omega)$  in the reference phase, i.e.,

$$\mathbf{E}_0(\mathbf{x}) = \tilde{\mathbf{E}}_0 \exp(i(\mathbf{k}_I(\omega) \cdot \mathbf{x} - \omega t)). \quad (\text{S23})$$

The associated wavelength  $\lambda = 2\pi/|\mathbf{k}_I|$  must lie between the inhomogeneity length scales  $\ell$  and the specimen size  $L$ . Granting that the effective-medium description is valid for the composite, we obtain the corresponding dielectric constant tensor  $\epsilon_e(\omega, \mathbf{k}_I)$ .

In the ensuing derivation, we make the following three assumptions on the phase properties:

- (a) the reference phase and phases 1, 2 are perfect insulators and dissipationless so that  $\epsilon_i$ s are purely real-valued and frequency-independent [i.e.,  $\epsilon_i(\omega) = \epsilon_i$  and  $\text{Im}[\epsilon_i] = 0$  for  $i = 1, 2, I$ ];

- (b) the dielectric constant of the reference phase is isotropic, i.e.,  $\boldsymbol{\varepsilon}_I = \varepsilon_I \mathbf{I}$ ; and
- (c) the magnetic permeability tensors of all phases are identical (i.e.,  $\boldsymbol{\mu}_1 = \boldsymbol{\mu}_2 = \boldsymbol{\mu}_I = \mu_0 \mathbf{I}$ ), where  $\mu_0$  is the magnetic permeability of vacuum.

The assumptions (a) and (b) imply the linear dispersion relation in the reference phase [i.e.,  $k_I(\omega) \equiv |\mathbf{k}_I(\omega)| = \sqrt{\varepsilon_I} \omega / c$ ], where  $c$  is the speed of light in vacuum, and thus we henceforth do not explicitly indicate the dependence of functions on  $\omega$ . We derive some important integral equations for local fields in Sec. II A. We derive a nonlocal homogenized relation associated with the strong-contrast expansions, equivalent to the standard constitutive relation in Sec. II B. We then derive the strong-contrast expansions for an arbitrarily-shaped exclusion region and any reference phase in Sec. II C. In Sec. II D, we then simplify the expansions derived in Sec. II C by assuming a spherical exclusion region and reference phase  $q$  ( $= 1, 2$ ).

### A. Integral Equation for Cavity Electric field

We derive the equation of motion for the electric field inside a composite at a given angular frequency  $\omega$ . For this purpose, we begin with the governing frequency-dependent wave equation that is obtained from the Maxwell equations and assumptions (a) and (c):

$$\nabla \times \nabla \times \mathbf{E}(\mathbf{x}) - \omega^2 \mu_0 \varepsilon_0 [\boldsymbol{\varepsilon}(\mathbf{x}) \cdot \mathbf{E}(\mathbf{x})] = 0,$$

where we have used separation of variables  $\mathbf{E}(\mathbf{x}, t) \rightarrow \mathbf{E}(\mathbf{x}) e^{-i\omega t}$ ,  $\mu_0$  is the magnetic permeability of vacuum, and  $\varepsilon_0$  is the dielectric permittivity of vacuum. We rewrite this homogeneous differential equation with respect to the reference phase as follows:

$$\nabla \times \nabla \times \mathbf{E}(\mathbf{x}) - \omega^2 \mu_0 \varepsilon_0 [\boldsymbol{\varepsilon}_I \cdot \mathbf{E}(\mathbf{x})] = \omega^2 \mu_0 \varepsilon_0 \mathbf{P}(\mathbf{x}), \quad (\text{S24})$$

where  $\mathbf{P}(\mathbf{x})$  is the *induced flux polarization field* given by

$$\mathbf{P}(\mathbf{x}) \equiv [\boldsymbol{\varepsilon}(\mathbf{x}) - \boldsymbol{\varepsilon}_I] \cdot \mathbf{E}(\mathbf{x}). \quad (\text{S25})$$

Assuming the isotropy of the reference phase, one can simplify Eq. (S24)

$$\nabla \times \nabla \times \mathbf{E}(\mathbf{x}) - k_I^2 \mathbf{E}(\mathbf{x}) = \left(\frac{\omega}{c}\right)^2 \mathbf{P}(\mathbf{x}), \quad (\text{S26})$$

where  $k_I \equiv \omega \sqrt{\varepsilon_I \varepsilon_0 \mu_0} = \sqrt{\varepsilon_I} \omega / c$  is the wavenumber of electromagnetic waves inside the reference phase.

When external electric field  $\mathbf{E}_0(\mathbf{x})$  is incident to the composite, the consequent local electric field  $\mathbf{E}(\mathbf{x})$  can be computed by using the dyadic Green's function  $\mathbf{G}^{(I)}(\mathbf{x}, \mathbf{x}')$  satisfying the following equation:

$$\begin{aligned} \nabla \times \nabla \times \mathbf{G}^{(I)}(\mathbf{x}, \mathbf{x}') - k_I^2 \mathbf{G}^{(I)}(\mathbf{x}, \mathbf{x}') &= \left(\frac{\omega}{c}\right)^2 \mathbf{I} \delta(\mathbf{x} - \mathbf{x}'), \\ \mathbf{G}^{(I)}(\mathbf{x}, \mathbf{x}') &\rightarrow 0, \quad |\mathbf{x}' - \mathbf{x}| \rightarrow \infty. \end{aligned} \quad (\text{S27})$$

Using the Green's method, the local electric field is written as

$$\mathbf{E}(\mathbf{x}) = \mathbf{E}_0(\mathbf{x}) + \int \mathbf{G}^{(I)}(\mathbf{x}, \mathbf{x}') \cdot \mathbf{P}(\mathbf{x}') d\mathbf{x}', \quad (\text{S28})$$

$$= \mathbf{E}_0(\mathbf{x}) + \underbrace{\int_{\text{inside the exclusion-region}} -\mathbf{D}^{(I)} \cdot \mathbf{P}(\mathbf{x})}_{\text{inside the exclusion-region}} + \underbrace{\int_{\text{outside the exclusion-region}} \mathbf{H}^{(I)}(\mathbf{x}, \mathbf{x}') \cdot \mathbf{P}(\mathbf{x}') d\mathbf{x}'}_{\text{outside the exclusion-region}}, \quad (\text{S29})$$

where we note that due to the singular nature of Green's function around the origin (i.e.,  $\mathbf{x} - \mathbf{x}' = \mathbf{0}$ ), the integral (S28) should be separated into two parts; one is the integral inside an infinitesimal exclusion region around the origin, and another is the integral outside the exclusion region (denoted by  $\int_{\epsilon} d\mathbf{x}'$ ). Thus, the Green's function can be written concisely as

$$\mathbf{G}^{(I)}(\mathbf{x}, \mathbf{x}') = -\mathbf{D}^{(I)} \delta(\mathbf{x} - \mathbf{x}') + \mathbf{H}^{(I)}(\mathbf{x} - \mathbf{x}'), \quad (\text{S30})$$

where the second-rank constant tensor  $\mathbf{D}^{(I)}$  depends on the shape of exclusion region. For a spherical exclusion region in  $\mathbb{R}^d$ ,

$$\mathbf{D}^{(I)} = \frac{1}{d\varepsilon_I} \mathbf{I}, \quad (\text{S31})$$

where  $\mathbf{I}$  is the second-rank identity tensor.

It is useful to provide explicit formulas for Eq. (S30) in both direct- and Fourier-space representations. In the direct-space representation (outside the “exclusion region”), the second-rank tensor field  $\mathbf{H}^{(I)}(\mathbf{r})$ , where  $\mathbf{r} \equiv \mathbf{x} - \mathbf{x}'$ , is given by

$$H_{ij}^{(I)}(\mathbf{r}) = i \frac{\pi}{2\varepsilon_I} \left( \frac{k_I}{2\pi r} \right)^{d/2} \left\{ \left[ k_I r \mathcal{H}_{d/2-1}^{(1)}(k_I r) - \mathcal{H}_{d/2}^{(1)}(k_I r) \right] \delta_{ij} + k_I r \mathcal{H}_{d/2+1}^{(1)}(k_I r) \hat{\mathbf{r}}_i \hat{\mathbf{r}}_j \right\} \quad (\text{S32})$$

$$= \begin{cases} \frac{i}{4\varepsilon_I} \left\{ \left[ k_I^2 \mathcal{H}_0^{(1)}(k_I r) - \frac{k_I}{r} \mathcal{H}_1^{(1)}(k_I r) \right] \delta_{ij} + k_I^2 \mathcal{H}_2^{(1)}(k_I r) \hat{\mathbf{r}}_i \hat{\mathbf{r}}_j \right\}, & d = 2 \\ \frac{\exp(ik_I r)}{\varepsilon_I 4\pi r^3} \left\{ [-1 + ik_I r + (k_I r)^2] \delta_{ij} + [3 - 3ik_I r - (k_I r)^2] \hat{\mathbf{r}}_i \hat{\mathbf{r}}_j \right\}, & d = 3 \end{cases} \quad (\text{S33})$$

where  $\hat{\mathbf{r}} \equiv \mathbf{r}/|\mathbf{r}|$  is a unit vector directed to  $\mathbf{r}$ , and  $\mathcal{H}_\nu^{(1)}(x)$  is the Hankel function of the first kind of order  $\nu$ . The Fourier representation of Eq. (S30), however, is concise and simple:

$$\tilde{G}_{ij}^{(I)}(\mathbf{q}) = \frac{1}{\varepsilon_I} \frac{k_I^2 \delta_{ij} - q_i q_j}{q^2 - k_I^2}, \quad (\text{S34})$$

which can be obtained from the Fourier transform of Eq. (S27) by using the orthogonality of two tensors  $\mathbf{\Pi} \equiv \mathbf{q}\mathbf{q}/|\mathbf{q}|^2$  and  $\mathbf{I} - \mathbf{\Pi}$ . It is important to note that Eq. (S34) is independent of the “exclusion region.”

We now express the integral equation (S29) more compactly in a linear operator form

$$\mathbf{E} = \mathbf{E}_0 + \mathbf{G}^{(I)} \mathbf{P}. \quad (\text{S35})$$

Excluding the contribution from a exclusion region in Eq. (S29), we obtain the integral equation for the *cavity intensity field*  $\mathbf{F}(\mathbf{x})$ :

$$\mathbf{F} \equiv \mathbf{E} + \mathbf{D}^{(I)} \cdot \mathbf{P} \quad (\text{S36})$$

$$= \mathbf{E}_0 + \mathbf{H}^{(I)} \mathbf{P} \quad (\text{S37})$$

$$= [\mathbf{I} + \mathbf{D}^{(I)} \cdot (\varepsilon(\mathbf{x}) - \varepsilon_I)] \cdot \mathbf{E}. \quad (\text{S38})$$

Using the definition (S25) and expression (S38), one obtains a linear constitutive relation between  $\mathbf{P}(\mathbf{x})$  and  $\mathbf{F}(\mathbf{x})$ :

$$\mathbf{P}(\mathbf{x}) = \mathbf{L}^{(I)}(\mathbf{x}) \cdot \mathbf{F}(\mathbf{x}), \quad (\text{S39})$$

where

$$\mathbf{L}^{(I)}(\mathbf{x}) = (\varepsilon(\mathbf{x}) - \varepsilon_I) \cdot [\mathbf{I} + \mathbf{D}^{(I)} \cdot (\varepsilon(\mathbf{x}) - \varepsilon_I)]^{-1} = \mathbf{L}_1^{(I)} \mathcal{I}^{(1)}(\mathbf{x}) + \mathbf{L}_2^{(I)} \mathcal{I}^{(2)}(\mathbf{x}), \quad (\text{S40})$$

and, for phase  $p$  ( $=1,2$ ),

$$\mathbf{L}_p^{(I)} \equiv (\varepsilon_p - \varepsilon_I) \cdot [\mathbf{I} + \mathbf{D}^{(I)} \cdot (\varepsilon_p - \varepsilon_I)]^{-1}. \quad (\text{S41})$$

#### Remarks:

1. The definition of  $\mathbf{G}^{(I)}(\mathbf{x}, \mathbf{x}')$ , given in Eq. (S27), is different from that given in Ref. [1]. Specifically, the Green's function in this work (S30) is a multiplication of that in Ref. [1] with  $(\omega/c)^2$ . By doing so, Eq. (S30) converges to its static counterpart in the static limit (i.e.,  $\omega \rightarrow 0$ ).
2. The reference phase  $I$  employed in the Green's function  $\mathbf{G}^{(I)}(\mathbf{x}, \mathbf{x}')$  can be different from phases 1 and 2. In the main text, however, we take phase  $q$  ( $=1,2$ ) as the reference phase for simplicity.

3. The general expression for the constant tensor  $\mathbf{D}^{(I)}$ , when a spheroidal-shaped exclusion region in three dimensions is chosen to be aligned with the  $+x$  direction, is given as [2, 3]

$$\mathbf{D}^{(I)} = \frac{1}{\varepsilon_I} [A^* \hat{\mathbf{x}} \hat{\mathbf{x}} + (1 - 2A^*)(\mathbf{I} - \hat{\mathbf{x}} \hat{\mathbf{x}})], \quad (\text{S42})$$

where  $A^*$  lies in the closed interval  $[0, 1/2]$ , and  $\hat{\mathbf{x}}$  is a unit vector along the  $x$  axis. For the three limit cases (i.e., sphere, disk-like, and needle-like), Eq. (S42) is written as

$$\mathbf{D}^{(I)} = \begin{cases} \frac{1}{3\varepsilon_I} \mathbf{I}, & \text{spherical} \\ \frac{1}{\varepsilon_I} \hat{\mathbf{x}} \hat{\mathbf{x}}, & \text{disk-like} \\ \frac{1}{2\varepsilon_I} (\mathbf{I} - \hat{\mathbf{x}} \hat{\mathbf{x}}), & \text{needle-like} \end{cases}. \quad (\text{S43})$$

The choice of the nonspherical exclusion-region shapes leads to expansion parameters different from that for the spherical exclusion region, which is primarily considered in the main article. Under the assumption that the dielectric constants of the polarized and reference phases are isotropic, these tensorial expansion parameters are obtained by substituting Eq. (S43) to Eq. (S41) as follows:

$$\frac{\mathbf{L}_p^{(I)}}{3\varepsilon_I} = \begin{cases} \frac{\varepsilon_p - \varepsilon_I}{3\varepsilon_p} \hat{\mathbf{x}} \hat{\mathbf{x}} + \frac{\varepsilon_p - \varepsilon_I}{3\varepsilon_I} (\mathbf{I} - \hat{\mathbf{x}} \hat{\mathbf{x}}), & \text{disk-like} \\ \frac{\varepsilon_p - \varepsilon_I}{3\varepsilon_I} \hat{\mathbf{x}} \hat{\mathbf{x}} + \frac{2}{3} \frac{\varepsilon_p - \varepsilon_I}{\varepsilon_p + \varepsilon_I} (\mathbf{I} - \hat{\mathbf{x}} \hat{\mathbf{x}}), & \text{needle-like} \end{cases}. \quad (\text{S44})$$

The resulting series expansions that apply to macroscopically anisotropic media are expected to have fast convergence properties for classes of microstructures different from the Hashin-Shtrikman coated-spheres structures. For the disk-like and needle-like cases, these structures correspond to stratified media and transversely isotropic media, respectively. The isotropic versions of these expansion parameters and the corresponding series expansions for macroscopically isotropic media are discussed in Appendix A in the main article.

4. Equation (S30) can be written more explicitly as

$$\mathbf{G}^{(I)}(\mathbf{x}, \mathbf{x}') = \begin{cases} -\mathbf{D}^{(I)} \delta(\mathbf{x} - \mathbf{x}'), & \text{outside the exclusion-region} \\ \mathbf{H}^{(I)}(\mathbf{x} - \mathbf{x}'), & \text{inside the exclusion-region.} \end{cases}$$

Due to this definition, while  $\mathbf{H}^{(I)}(\mathbf{r})$  in the direct-space is independent of a choice of exclusion-region, the Fourier transform  $\tilde{\mathbf{H}}^{(I)}(\mathbf{q})$  depends on the shape of the exclusion region

$$\begin{aligned} \tilde{\mathbf{H}}^{(I)}(\mathbf{q}) &= \int d\mathbf{r} e^{-i\mathbf{q} \cdot \mathbf{r}} \mathbf{H}^{(I)}(\mathbf{r}) = \int_{\epsilon} d\mathbf{r} e^{-i\mathbf{q} \cdot \mathbf{r}} \mathbf{H}^{(I)}(\mathbf{r}) \\ &= \tilde{\mathbf{G}}^{(I)}(\mathbf{q}) + \mathbf{D}^{(I)}, \end{aligned} \quad (\text{S45})$$

where we have used Eq. (S30).

## B. Equivalence of Two Nonlocal Relations

In the nonlocal strong-contrast formalism, the following nonlocal homogenized constitutive relation is employed:

$$\widetilde{\langle \mathbf{P} \rangle}(\mathbf{k}) = \mathbf{L}_e^{(I)}(\mathbf{k}) \cdot \widetilde{\langle \mathbf{F} \rangle}(\mathbf{k}), \quad (\text{S46})$$

where the constant tensor  $\mathbf{L}_e^{(I)}(\mathbf{k})$  is written explicitly as

$$\mathbf{L}_e^{(I)}(\mathbf{k}) \equiv [\varepsilon_e(\mathbf{k}) - \varepsilon_I] \cdot \left[ \mathbf{I} + \mathbf{D}^{(I)} \cdot (\varepsilon_e(\mathbf{k}) - \varepsilon_I) \right]^{-1}. \quad (\text{S47})$$

Here,  $\mathbf{k}$  is a wavevector,  $\widetilde{\langle f \rangle}(\mathbf{k}) \equiv \int \langle f \rangle(\mathbf{x}) \exp(-i\mathbf{k} \cdot \mathbf{x}) d\mathbf{x}$ ,  $\langle f \rangle(\mathbf{x})$  is an ensemble average of field  $f(x)$  that varies with position. We note that a relation like Eq. (S46) is nonlocal in space because it is written in terms of a convolution operation

$$\langle \mathbf{P} \rangle(\mathbf{x}) = \int d\mathbf{x}' \mathbf{L}_e^{(I)}(\mathbf{x} - \mathbf{x}') \cdot \langle \mathbf{F} \rangle(\mathbf{x}'), \quad (\text{S48})$$

implying that  $\langle \mathbf{P} \rangle(\mathbf{x})$  at position  $\mathbf{x}$  is determined by  $\langle \mathbf{F} \rangle(\mathbf{x}')$  in vicinity of  $\mathbf{x}$ . In this subsection, we show that the relation (S46) is equivalent to the following popular constitutive relation:

$$\langle \widetilde{\mathbf{D}} \rangle(\mathbf{k}) = \varepsilon_0 \varepsilon_e(\mathbf{k}) \cdot \langle \widetilde{\mathbf{E}} \rangle(\mathbf{k}), \quad (\text{S49})$$

where  $\langle \widetilde{\mathbf{D}} \rangle(\mathbf{k})$  is the spatial Fourier transform of an ensemble average of the electric displacement field

$$\mathbf{D}(\mathbf{x}) \equiv \varepsilon_0 \mathbf{E}(\mathbf{x}) + \mathcal{P}(\mathbf{x}) = \varepsilon_0 \varepsilon(\mathbf{x}) \cdot \mathbf{E}(\mathbf{x}), \quad (\text{S50})$$

and  $\mathcal{P}(\mathbf{x})$  is the electric polarization density, which is different from  $\mathbf{P}(\mathbf{x})$  defined in Eq. (S25).

To do so, we rewrite the induced flux polarization field  $\langle \widetilde{\mathbf{P}} \rangle(\mathbf{k})$  and the cavity intensity field  $\langle \widetilde{\mathbf{F}} \rangle(\mathbf{k})$  in terms of  $\langle \widetilde{\mathbf{E}} \rangle(\mathbf{k})$ , and then eliminate  $\langle \widetilde{\mathbf{E}} \rangle(\mathbf{k})$  between these two expressions. We begin with expressions of the induced flux polarization field and cavity intensity field in terms of the electric displacement field  $\mathbf{D}(\mathbf{x})$  and electric field  $\mathbf{E}(\mathbf{x})$ . Using Eqs. (S25), (S36), and (S50), the followings are obtained

$$\mathbf{P}(\mathbf{x}) = \frac{1}{\varepsilon_0} \mathbf{D}(\mathbf{x}) - \varepsilon_I \mathbf{E}(\mathbf{x}), \quad (\text{S51})$$

$$\mathbf{F}(\mathbf{x}) = \mathbf{E}(\mathbf{x}) + \mathbf{D}^{(I)} \cdot \mathbf{P}(\mathbf{x}). \quad (\text{S52})$$

After averaging Eq. (S51) over an ensemble, taking its spatial Fourier transform, and substituting Eq. (S49) into it to eliminate  $\langle \widetilde{\mathbf{D}} \rangle(\mathbf{k})$ , we obtain the following expression

$$\begin{aligned} \langle \widetilde{\mathbf{P}} \rangle(\mathbf{k}) &= \langle \widetilde{\mathbf{D}} \rangle(\mathbf{k}) / \varepsilon_0 - \varepsilon_I \langle \widetilde{\mathbf{E}} \rangle(\mathbf{k}) \\ &= [\varepsilon_e(\mathbf{k}) - \varepsilon_I \mathbf{I}] \cdot \langle \widetilde{\mathbf{E}} \rangle(\mathbf{k}). \end{aligned} \quad (\text{S53})$$

Analogously, we re-express Eq. (S52) in terms of  $\langle \widetilde{\mathbf{E}} \rangle(\mathbf{k})$  by using Eq. (S53):

$$\begin{aligned} \langle \widetilde{\mathbf{F}} \rangle(\mathbf{k}) &= \langle \widetilde{\mathbf{E}} \rangle(\mathbf{k}) + \mathbf{D}^{(I)} \cdot \langle \widetilde{\mathbf{P}} \rangle(\mathbf{k}) \\ &= \left\{ \mathbf{I} + \mathbf{D}^{(I)} \cdot [\varepsilon_e(\mathbf{k}) - \varepsilon_I \mathbf{I}] \right\} \cdot \langle \widetilde{\mathbf{E}} \rangle(\mathbf{k}). \end{aligned} \quad (\text{S54})$$

Now, the linear relation (S46) is obtained by inverting the right-side of Eq. (S54) and substituting it to Eq. (S53). Later, we will show that the wavevector  $\mathbf{k}$  in Eq. (S46) is indeed identical to the wavevector of the incident waves  $\mathbf{k}_I$ .

### C. Strong-Contrast Expansion in General Cases

In this subsection, we derive an exact expression for the effective dielectric constant tensor  $\varepsilon_e$  for an arbitrary reference phase  $I$  ( $\neq 1, 2$ ) and an arbitrarily-shaped exclusion region. To do so, we derive an explicit expression for the constant tensor  $\mathbf{L}_e^{(I)}(\mathbf{k}_I)$  in the nonlocal homogenized relation (S48) with an incident electric field (S23).

For this purpose, we first find explicit expressions for  $\langle \widetilde{\mathbf{P}} \rangle(\mathbf{k})$  and  $\langle \widetilde{\mathbf{F}} \rangle(\mathbf{k})$  in terms of the applied field  $\tilde{\mathbf{E}}_0$  from the integral equation (S37). We then find an explicit expression for the effective constant tensor  $\mathbf{L}_e^{(I)}$  by eliminating  $\tilde{\mathbf{E}}_0$  between these two expressions. Keeping in mind that the tensors  $\mathbf{L}^{(I)}$ ,  $\mathbf{L}_e^{(I)}$ , and  $\mathbf{H}^{(I)}$  are associated with the reference phase  $I$ , we shall temporarily drop the superscript  $I$  when referring these tensors in the following derivation. Applying Eq. (S37) to Eq. (S39) yields

$$\mathbf{P} = \mathbf{L}\mathbf{E}_0 + \mathbf{L}\mathbf{H}\mathbf{P}. \quad (\text{S55})$$

Iterative substitution of this expression with the polarization field in the right-hand side gives

$$\mathbf{P} = (\mathbf{I} + \mathbf{L}\mathbf{H} + \mathbf{L}\mathbf{H}\mathbf{L}\mathbf{H} + \cdots) \mathbf{L}\mathbf{E}_0 = [\mathbf{I} - \mathbf{L}\mathbf{H}]^{-1} \mathbf{L}\mathbf{E}_0 = \mathbf{S}\mathbf{E}_0. \quad (\text{S56})$$

More explicitly, we write out Eq. (S56) as

$$\begin{aligned} \mathbf{P}(\mathbf{1}) &= \int_{\epsilon} d\mathbf{1}' \left[ \mathbf{L}(\mathbf{1}) \delta(\mathbf{1} - \mathbf{1}') + \mathbf{L}(\mathbf{1}) \mathbf{H}(\mathbf{1}, \mathbf{1}') \mathbf{L}(\mathbf{1}') \right. \\ &\quad \left. + \int_{\epsilon} d\mathbf{2} \mathbf{L}(\mathbf{1}) \mathbf{H}(\mathbf{1}, \mathbf{2}) \mathbf{L}(\mathbf{2}) \mathbf{H}(\mathbf{2}, \mathbf{1}') \mathbf{L}(\mathbf{1}') + \cdots \right] \cdot \mathbf{E}_0(\mathbf{1}'). \\ &= \int_{\epsilon} d\mathbf{1}' \mathbf{S}(\mathbf{1}, \mathbf{1}') \cdot \mathbf{E}_0(\mathbf{1}'), \end{aligned} \quad (\text{S57})$$

where  $\delta(\mathbf{x})$  is the Dirac delta function in  $\mathbb{R}^d$ , and boldface numbers  $\mathbf{1}', \mathbf{1}, \mathbf{2}, \dots$  are short-hand notations for position vectors  $\mathbf{r}_{1'}, \mathbf{r}_1, \mathbf{r}_2, \dots$ . The two-point tensor operator  $\mathbf{S}(\mathbf{1}, \mathbf{1}')$  explicitly reads

$$\mathbf{S}(\mathbf{1}, \mathbf{1}') = \mathbf{L}(\mathbf{1}) \delta(\mathbf{1} - \mathbf{1}') + \mathbf{L}(\mathbf{1}) \mathbf{H}(\mathbf{1}, \mathbf{1}') \mathbf{L}(\mathbf{1}') + \int_{\epsilon} d\mathbf{2} \mathbf{L}(\mathbf{1}) \mathbf{H}(\mathbf{1}, \mathbf{2}) \mathbf{L}(\mathbf{2}) \mathbf{H}(\mathbf{2}, \mathbf{1}') \mathbf{L}(\mathbf{1}') + \dots \quad (\text{S58})$$

For a statistically homogeneous medium, an ensemble average of the two-point operator  $\mathbf{S}(\mathbf{1}, \mathbf{1}')$  becomes dependent on relative positions, i.e.,  $\langle \mathbf{S} \rangle(\mathbf{1}, \mathbf{1}') = \langle \mathbf{S} \rangle(\mathbf{1} - \mathbf{1}')$ , and an ensemble average of Eq. (S57) can be written as a convolution:

$$\langle \mathbf{P} \rangle(\mathbf{1}) = \int_{\epsilon} d\mathbf{1}' \langle \mathbf{S} \rangle(\mathbf{1} - \mathbf{1}') \cdot \mathbf{E}_0(\mathbf{1}'). \quad (\text{S59})$$

The nonlocal relation (S59) can be simplified in the Fourier space as follows:

$$\widetilde{\langle \mathbf{P} \rangle}(\mathbf{k}) = \widetilde{\langle \mathbf{S} \rangle}(\mathbf{k}) \cdot \tilde{\mathbf{E}}_0(\mathbf{k}). \quad (\text{S60})$$

Here it is crucial to note that from Eq. (S23),

$$\tilde{\mathbf{E}}_0(\mathbf{k}) = \tilde{\mathbf{E}}_0 \delta(\mathbf{k} - \mathbf{k}_I), \quad (\text{S61})$$

implying that the wavevector  $\mathbf{k}$  in Eq. (S60) must be identical to  $\mathbf{k}_I$ . From Eq. (S58), the quantity  $\widetilde{\langle \mathbf{S} \rangle}(\mathbf{k}_I)$  is explicitly written as

$$\begin{aligned} \widetilde{\langle \mathbf{S} \rangle}(\mathbf{k}_I) &= \int d(\mathbf{1} - \mathbf{1}') e^{-i\mathbf{k}_I \cdot (\mathbf{1} - \mathbf{1}')} \left\langle \left[ \mathbf{L}(\mathbf{1}) \delta(\mathbf{1} - \mathbf{1}') + \mathbf{L}(\mathbf{1}) \mathbf{H}(\mathbf{1}, \mathbf{1}') \mathbf{L}(\mathbf{1}') \right. \right. \\ &\quad \left. \left. + \int_{\epsilon} d\mathbf{2} \mathbf{L}(\mathbf{1}) \mathbf{H}(\mathbf{1}, \mathbf{2}) \mathbf{L}(\mathbf{2}) \mathbf{H}(\mathbf{2}, \mathbf{1}') \mathbf{L}(\mathbf{1}') + \dots \right] \right\rangle \\ &= \int d(\mathbf{1} - \mathbf{1}') e^{-i\mathbf{k}_I \cdot (\mathbf{1} - \mathbf{1}')} \left[ \sum_{p_1=1}^2 \mathbf{L}_{p_1} \langle \mathcal{I}^{(p_1)}(\mathbf{1}) \rangle \delta(\mathbf{1} - \mathbf{1}') + \sum_{p_1, p_2=1}^2 \mathbf{L}_{p_1} \mathbf{H}(\mathbf{1} - \mathbf{1}') \mathbf{L}_{p_2} \langle \mathcal{I}^{(p_1)}(\mathbf{1}) \mathcal{I}^{(p_2)}(\mathbf{1}') \rangle \right. \\ &\quad \left. + \sum_{p_1, p_2, p_3=1}^2 \mathbf{L}_{p_1} \mathbf{H}(\mathbf{1} - \mathbf{2}) \mathbf{L}_{p_2} \mathbf{H}(\mathbf{2} - \mathbf{1}') \mathbf{L}_{p_3} \langle \mathcal{I}^{(p_1)}(\mathbf{1}) \mathcal{I}^{(p_2)}(\mathbf{2}) \mathcal{I}^{(p_3)}(\mathbf{1}') \rangle + \dots \right] \\ &= \mathbb{A}_1 + \mathbb{A}_2 + \mathbb{A}_3 + \dots, \end{aligned} \quad (\text{S62})$$

where

$$\mathbb{A}_1 = \langle \mathbf{L}(\mathbf{1}) \rangle = \phi_1 \mathbf{L}_1 + \phi_2 \mathbf{L}_2, \quad (\text{S64})$$

$$\mathbb{A}_2 = \sum_{p_1, p_2=1}^2 \int_{\epsilon} d(\mathbf{1} - \mathbf{2}) \mathbf{L}_{p_1} \mathbf{H}(\mathbf{1}, \mathbf{2}) e^{-i\mathbf{k}_I \cdot (\mathbf{1} - \mathbf{2})} \mathbf{L}_{p_2} \langle \mathcal{I}^{(p_1)}(\mathbf{1}) \mathcal{I}^{(p_2)}(\mathbf{2}) \rangle, \quad (\text{S65})$$

$$\begin{aligned} \mathbb{A}_3 &= \sum_{p_1, p_2, p_3=1}^2 \int_{\epsilon} d\mathbf{2} d(-\mathbf{3}) \mathbf{L}_{p_1} \mathbf{H}(\mathbf{1}, \mathbf{2}) e^{-i\mathbf{k}_I \cdot (\mathbf{1} - \mathbf{2})} \mathbf{L}_{p_2} \mathbf{H}(\mathbf{2}, \mathbf{3}) e^{-i\mathbf{k}_I \cdot (\mathbf{2} - \mathbf{3})} \mathbf{L}_{p_3} \\ &\quad \times \langle \mathcal{I}^{(p_1)}(\mathbf{1}) \mathcal{I}^{(p_2)}(\mathbf{2}) \mathcal{I}^{(p_3)}(\mathbf{3}) \rangle. \end{aligned} \quad (\text{S66})$$

We then obtain an expression for  $\langle \mathbf{F} \rangle(\mathbf{1})$  from an ensemble average of Eq. (S37):

$$\langle \mathbf{F} \rangle(\mathbf{1}) = \mathbf{E}_0(\mathbf{1}) + \int_{\epsilon} d\mathbf{2} \mathbf{H}(\mathbf{1} - \mathbf{2}) \cdot \langle \mathbf{P} \rangle(\mathbf{2}). \quad (\text{S67})$$

Its spatial Fourier transform gives

$$\begin{aligned} \widetilde{\langle \mathbf{F} \rangle}(\mathbf{k}_I) &= \tilde{\mathbf{E}}_0(\mathbf{k}_I) + \tilde{\mathbf{H}}(\mathbf{k}_I) \cdot \widetilde{\langle \mathbf{P} \rangle}(\mathbf{k}_I) \\ &= \left[ \widetilde{\langle \mathbf{S} \rangle}(\mathbf{k}_I)^{-1} + \tilde{\mathbf{H}}(\mathbf{k}_I) \right] \cdot \widetilde{\langle \mathbf{P} \rangle}(\mathbf{k}_I), \end{aligned} \quad (\text{S68})$$

where we have eliminated the term  $\tilde{\mathbf{E}}_0(\mathbf{k}_I)$  by substituting Eq. (S60). Eventually, comparing the above expression to Eq. (S46) gives an expression of the constant tensor  $\mathbf{L}_e$  at given frequency  $\omega$  and wavevector  $\mathbf{k}_I$ :

$$\begin{aligned} [\mathbf{L}_e(\mathbf{k}_I)]^{-1} &= \widetilde{(\mathbf{S})}(\mathbf{k}_I)^{-1} + \tilde{\mathbf{H}}(\mathbf{k}_I) \\ &= [\mathbf{I} + \mathbf{D} \cdot (\boldsymbol{\varepsilon}_e(\mathbf{k}_I) - \boldsymbol{\varepsilon}_I \mathbf{I})] \cdot [\boldsymbol{\varepsilon}_e(\mathbf{k}_I) - \boldsymbol{\varepsilon}_I \mathbf{I}]^{-1}, \end{aligned} \quad (\text{S69})$$

where we have employed Eq. (S47). More explicitly, Eq. (S69) reads

$$\begin{aligned} [\mathbf{L}_e(\mathbf{k}_I)]^{-1} &= \left[ \bigcircled{\mathbb{A}_1} + \bigcircled{\mathbb{A}_2} + \bigcircled{\mathbb{A}_3} + \cdots \right]^{-1} + \int_{\epsilon} d(-\mathbf{2}) \mathbf{H}(\mathbf{1} - \mathbf{2}) e^{-i\mathbf{k}_I \cdot (\mathbf{1} - \mathbf{2})} \\ &= \bigcircled{\mathbb{A}_1}^{-1} \left[ \mathbf{I} + \bigcircled{\mathbb{A}_2} \bigcircled{\mathbb{A}_1}^{-1} + \bigcircled{\mathbb{A}_3} \bigcircled{\mathbb{A}_1}^{-1} + \cdots \right]^{-1} + \int_{\epsilon} d(-\mathbf{2}) \mathbf{H}(\mathbf{1} - \mathbf{2}) e^{-i\mathbf{k}_I \cdot (\mathbf{1} - \mathbf{2})} \end{aligned} \quad (\text{S70})$$

$$\begin{aligned} &= \bigcircled{\mathbb{A}_1}^{-1} \left[ \mathbf{I} - \left( \bigcircled{\mathbb{A}_2} \bigcircled{\mathbb{A}_1}^{-1} + \bigcircled{\mathbb{A}_3} \bigcircled{\mathbb{A}_1}^{-1} + \cdots \right) + \left( \bigcircled{\mathbb{A}_2} \bigcircled{\mathbb{A}_1}^{-1} + \bigcircled{\mathbb{A}_3} \bigcircled{\mathbb{A}_1}^{-1} + \cdots \right)^2 \right. \\ &\quad \left. + \cdots \right] + \int_{\epsilon} d(\mathbf{1} - \mathbf{2}) \mathbf{H}(\mathbf{1} - \mathbf{2}) e^{-i\mathbf{k}_I \cdot (\mathbf{1} - \mathbf{2})}, \end{aligned} \quad (\text{S71})$$

where  $\bigcircled{\mathbb{A}_1}$ ,  $\bigcircled{\mathbb{A}_2}$ , and  $\bigcircled{\mathbb{A}_3}$  are given in Eqs. (S64), (S65), and (S66), respectively.

Expression (S71) can be rewritten as

$$\begin{aligned} \langle \mathbf{L}(\mathbf{1}) \rangle \cdot [\mathbf{L}_e(\mathbf{k}_I)]^{-1} \cdot \langle \mathbf{L}(\mathbf{1}) \rangle &= \langle \mathbf{L}(\mathbf{1}) \rangle \cdot \left\{ [\boldsymbol{\varepsilon}_e(\mathbf{k}_I) - \boldsymbol{\varepsilon}_I \mathbf{I}] \cdot [\mathbf{I} + \mathbf{D} \cdot (\boldsymbol{\varepsilon}_e(\mathbf{k}_I) - \boldsymbol{\varepsilon}_I \mathbf{I})]^{-1} \right\}^{-1} \cdot \langle \mathbf{L}(\mathbf{1}) \rangle \\ &= \langle \mathbf{L}(\mathbf{1}) \rangle - \underbrace{\left[ \bigcircled{\mathbb{A}_2} - \bigcircled{\mathbb{A}_1} \int_{\epsilon} d(-\mathbf{2}) \mathbf{H}(\mathbf{1} - \mathbf{2}) e^{-i\mathbf{k}_I \cdot (\mathbf{1} - \mathbf{2})} \bigcircled{\mathbb{A}_1} \right]}_{\equiv \mathbf{A}_2^{(p)}(\mathbf{k}_I) \cdot (\mathbf{L}_2 - \mathbf{L}_1)^2 / (d\varepsilon_I)} \\ &\quad - \underbrace{\left[ \bigcircled{\mathbb{A}_3} - \bigcircled{\mathbb{A}_2} \bigcircled{\mathbb{A}_1}^{-1} \bigcircled{\mathbb{A}_2} \right]}_{\equiv \mathbf{A}_3^{(p)}(\mathbf{k}_I) \cdot (\mathbf{L}_2 - \mathbf{L}_1)^3 / (d\varepsilon_I)^2} + \cdots \\ &= \langle \mathbf{L}(\mathbf{1}) \rangle - \sum_{n=2}^{\infty} \mathbf{A}_n^{(p)}(\mathbf{k}_I) \cdot (\mathbf{L}_2 - \mathbf{L}_1)^n / (d\varepsilon_I)^{n-1}, \end{aligned} \quad (\text{S72})$$

where  $\mathbf{T}^n$  stands for  $n$  successive inner products of a second-rank tensor  $\mathbf{T}$ . Using the following identity

$$\langle \mathcal{I}^{(p_1)}(\mathbf{1}) \mathcal{I}^{(p_2)}(\mathbf{2}) \rangle - \langle \mathcal{I}^{(p_1)}(\mathbf{1}) \rangle \langle \mathcal{I}^{(p_2)}(\mathbf{2}) \rangle = \begin{cases} \chi_V(\mathbf{1} - \mathbf{2}), & p_1 = p_2 \\ -\chi_V(\mathbf{1} - \mathbf{2}), & p_1 \neq p_2 \end{cases},$$

we simplify the second-order term as follows:

$$\begin{aligned} \mathbf{A}_2^{(p)}(\mathbf{k}_I) (\mathbf{L}_2 - \mathbf{L}_1)^2 / (d\varepsilon_I) &\equiv \bigcircled{\mathbb{A}_2} - \bigcircled{\mathbb{A}_1} \int_{\epsilon} d(\mathbf{1} - \mathbf{2}) \mathbf{H}(\mathbf{1} - \mathbf{2}) e^{-i\mathbf{k}_I \cdot (\mathbf{1} - \mathbf{2})} \bigcircled{\mathbb{A}_1} \\ &= \sum_{p_1, p_2=1}^2 \int_{\epsilon} d(\mathbf{1} - \mathbf{2}) \mathbf{L}_{p_1} \cdot \mathbf{H}(\mathbf{1} - \mathbf{2}) e^{-i\mathbf{k}_I \cdot (\mathbf{1} - \mathbf{2})} \cdot \mathbf{L}_{p_2} \left[ \langle \mathcal{I}^{(p_1)}(\mathbf{1}) \mathcal{I}^{(p_2)}(\mathbf{2}) \rangle - \langle \mathcal{I}^{(p_1)}(\mathbf{1}) \rangle \langle \mathcal{I}^{(p_2)}(\mathbf{2}) \rangle \right] \\ &= \int_{\epsilon} d(\mathbf{1} - \mathbf{2}) (\mathbf{L}_2 - \mathbf{L}_1) \cdot \mathbf{H}(\mathbf{1} - \mathbf{2}) e^{-i\mathbf{k}_I \cdot (\mathbf{1} - \mathbf{2})} \cdot (\mathbf{L}_2 - \mathbf{L}_1) \chi_V(\mathbf{1} - \mathbf{2}), \end{aligned} \quad (\text{S73})$$

$$\begin{aligned} \mathbf{A}_3^{(p)}(\mathbf{k}_I) (\mathbf{L}_2 - \mathbf{L}_1)^3 / (d\varepsilon_I)^2 &\equiv \bigcircled{\mathbb{A}_3} - \bigcircled{\mathbb{A}_2} \bigcircled{\mathbb{A}_1}^{-1} \bigcircled{\mathbb{A}_2} \\ &= \sum_{p_1, p_2, p_3=1}^2 \int_{\epsilon} d\mathbf{1} d\mathbf{2} \mathbf{L}_{p_1} \cdot \mathbf{H}(\mathbf{1} - \mathbf{2}) e^{-i\mathbf{k}_I \cdot (\mathbf{1} - \mathbf{2})} \cdot \mathbf{L}_{p_2} \cdot \mathbf{H}(\mathbf{2} - \mathbf{3}) e^{-i\mathbf{k}_I \cdot (\mathbf{2} - \mathbf{3})} \cdot \mathbf{L}_{p_3} \langle \mathcal{I}^{(p_1)}(\mathbf{1}) \mathcal{I}^{(p_2)}(\mathbf{2}) \mathcal{I}^{(p_3)}(\mathbf{3}) \rangle \\ &\quad - \sum_{p_1, p_2, p_3, p_4=1}^2 \int_{\epsilon} d\mathbf{1} \left[ \mathbf{L}_{p_1} \cdot \mathbf{H}(\mathbf{1} - \mathbf{2}) e^{-i\mathbf{k}_I \cdot (\mathbf{1} - \mathbf{2})} \cdot \mathbf{L}_{p_2} \langle \mathcal{I}^{(p_1)}(\mathbf{1}) \mathcal{I}^{(p_2)}(\mathbf{2}) \rangle \right] \cdot \langle \mathbf{L}(\mathbf{2}) \rangle^{-1} \\ &\quad \cdot \int_{\epsilon} d\mathbf{2} \left[ \mathbf{L}_{p_3} \cdot \mathbf{H}(\mathbf{2} - \mathbf{3}) e^{-i\mathbf{k}_I \cdot (\mathbf{2} - \mathbf{3})} \cdot \mathbf{L}_{p_4} \langle \mathcal{I}^{(p_3)}(\mathbf{2}) \mathcal{I}^{(p_4)}(\mathbf{3}) \rangle \right]. \end{aligned} \quad (\text{S74})$$

Note that it is highly nontrivial to simplify the  $n$ -th order term because the inner products of  $\langle \mathbf{L}(\mathbf{1}) \rangle^{-1}$  and other tensors are generally non-commutable.

**Remarks:**

1. In principle, the effective dielectric constant tensor  $\boldsymbol{\varepsilon}_e$  in the full exact expansion (S72) is independent of the choice of reference phase.
2. It is important to note that in the original local strong-contrast expansions [1] that applies to the quastatic regime, the authors employed a local relation  $\langle \mathbf{P}(\mathbf{1}) \rangle = \langle \widetilde{\mathbf{S}} \rangle(\mathbf{k} = \mathbf{0}) \cdot \mathbf{E}_0(\mathbf{1})$ , implying that electric polarization at one position is determined solely by the electric field at that position. Therefore, one would not expect the original strong-contrast approximations to provide good estimates for relatively large wavelengths. When the wavelength is comparable or smaller than the inhomogeneity length scales  $\ell$ , however, the electric polarization  $\mathbf{P}$  at one position  $\mathbf{1}$  is determined by the electric field at a different position (nonlocality). Since the constitutive relation (S59) takes such spatial dispersion effects into account [4, 5], the nonlocal strong-contrast approximation derived here gives more accurate estimates from long- to intermediate-wavelength regime.
3. The tensor operator  $\mathbf{S}$  defined in Eq. (S56) is formally similar to the scattering operator  $\mathcal{T}$  that arises in standard multiple scattering theory [6–9]. However,  $\mathbf{S}$  can be regarded to be a “generalized scattering operator” with superior mathematical properties compared to  $\mathcal{T}$ ; see Sec. IX.

#### D. Expansions for the spherical exclusion region

In this subsection, we derive the strong-contrast expansions that are presented in the main text. Specifically, we make two additional assumptions to simplify expansions (S72) in Sec. II C: the reference phase is taken to be one phase  $q$  of the composite [i.e.,  $I = q$  ( $= 1, 2$ )]; and the exclusion region is spherical. Then, we have simplified expressions for some tensor quantities:

$$\mathbf{D}^{(I)} \rightarrow \mathbf{D}^{(q)} = \frac{1}{d\varepsilon_q} \mathbf{I}, \quad (\text{S75})$$

$$\tilde{H}_{ij}^{(I)}(\mathbf{q}) \rightarrow \frac{q^2 \delta_{ij} - q_i q_j + (d-1)k_q^2 \delta_{ij}}{d\varepsilon_q(q^2 - k_q^2)}, \quad (\text{S76})$$

$$\mathbf{L}_{p_1}^{(I)} \rightarrow \begin{cases} \mathbf{L}^{(q)} \equiv d\varepsilon_q \beta_{pq} \mathbf{I}, & p_1 \neq q \\ \mathbf{0}, & p_1 = q \end{cases}, \quad (\text{S77})$$

$$\langle \mathbf{L}^{(I)}(\mathbf{1}) \rangle \rightarrow \phi_p \mathbf{L}^{(q)} \quad (q \neq p). \quad (\text{S78})$$

Similarly, the nonlocal relation (S68) is written as

$$\langle \widetilde{\mathbf{F}} \rangle(\mathbf{k}_q) = [\mathbf{L}_e(\mathbf{k}_q)]^{-1} \cdot \langle \widetilde{\mathbf{P}} \rangle(\mathbf{k}_q), \quad (\text{S79})$$

where

$$\begin{aligned} [\mathbf{L}_e(\mathbf{k}_q)]^{-1} &= \langle \widetilde{\mathbf{S}} \rangle(\mathbf{k}_q)^{-1} + \tilde{\mathbf{H}}(\mathbf{k}_q) \\ &= \left\{ [\boldsymbol{\varepsilon}_e(\mathbf{k}_q) - \varepsilon_q \mathbf{I}] \cdot [\boldsymbol{\varepsilon}_e(\mathbf{k}_q) + (d-1)\varepsilon_q \mathbf{I}]^{-1} \right\}^{-1}. \end{aligned} \quad (\text{S80})$$

To solve Eq. (S80), we first simplify the expression for  $\langle \widetilde{\mathbf{S}} \rangle(\mathbf{k}_q)^{-1}$ . Substituting Eqs. (S76)-(S78) to the Fourier

transform of  $\langle \mathbf{S} \rangle (\mathbf{1} - \mathbf{1}')$  given in (S62) leads to

$$\begin{aligned}
\widetilde{\langle \mathbf{S} \rangle}(\mathbf{k}_q) &= \int d(\mathbf{1} - \mathbf{1}') e^{-i\mathbf{k}_q \cdot (\mathbf{1} - \mathbf{1}')} \left\langle \left[ L(\mathbf{1}) \delta(\mathbf{1} - \mathbf{1}') + L(\mathbf{1}) \mathbf{H}(\mathbf{1}, \mathbf{1}') L(\mathbf{1}') \right. \right. \\
&\quad \left. \left. + \int_{\epsilon} d\mathbf{2} L(\mathbf{1}) \mathbf{H}(\mathbf{1}, \mathbf{2}) L(\mathbf{2}) \mathbf{H}(\mathbf{2}, \mathbf{1}') L(\mathbf{1}') + \dots \right] \right\rangle \\
&= \int d(\mathbf{1} - \mathbf{1}') e^{-i\mathbf{k}_q \cdot (\mathbf{1} - \mathbf{1}')} \left[ \phi_p (d\varepsilon_q \beta_{pq} \mathbf{I}) \delta(\mathbf{1} - \mathbf{1}') + (d\varepsilon_q \beta_{pq})^2 \mathbf{H}(\mathbf{1} - \mathbf{1}') S_2^{(p)}(\mathbf{1} - \mathbf{1}') \right. \\
&\quad \left. + \int_{\epsilon} d\mathbf{2} (d\varepsilon_q \beta_{pq})^3 \mathbf{H}(\mathbf{1} - \mathbf{2}) \cdot \mathbf{H}(\mathbf{2} - \mathbf{1}') \cdot S_3^{(p)}(\mathbf{1} - \mathbf{1}', \mathbf{2} - \mathbf{1}') + \dots \right] \\
&= \phi_p (d\varepsilon_q \beta_{pq} \mathbf{I}) + (d\varepsilon_q \beta_{pq})^2 \int d\mathbf{x}_1 \mathbf{H}(\mathbf{x}_1 - \mathbf{x}_2) e^{-i\mathbf{k}_q \cdot (\mathbf{x}_1 - \mathbf{x}_2)} S_2^{(p)}(\mathbf{x}_1 - \mathbf{x}_2) \\
&\quad + (d\varepsilon_q \beta_{pq})^3 \int d\mathbf{x}_1 d\mathbf{x}_2 \mathbf{H}(\mathbf{x}_1 - \mathbf{x}_2) e^{-i\mathbf{k}_q \cdot (\mathbf{x}_1 - \mathbf{x}_2)} \cdot \mathbf{H}(\mathbf{x}_2 - \mathbf{x}_3) e^{-i\mathbf{k}_q \cdot (\mathbf{x}_2 - \mathbf{x}_3)} S_3^{(p)}(\mathbf{x}_1, \mathbf{x}_2, \mathbf{x}_3) \\
&\quad + \sum_{n=4}^{\infty} \mathbb{A}_n, \tag{S81}
\end{aligned}$$

where we note that  $S_n^{(p)}(\mathbf{x}_1, \dots, \mathbf{x}_{n-1}, \mathbf{x}_n) = S_n^{(p)}(\mathbf{x}_1 - \mathbf{x}_n, \dots, \mathbf{x}_{n-1} - \mathbf{x}_n)$  due to statistical homogeneity, and

$$\begin{aligned}
\mathbb{A}_n &\equiv (d\varepsilon_q \beta_{pq})^n \int d\mathbf{x}_1 \dots d\mathbf{x}_{n-1} \mathbf{H}(\mathbf{x}_1 - \mathbf{x}_2) e^{-i\mathbf{k}_q \cdot (\mathbf{x}_1 - \mathbf{x}_2)} \dots \mathbf{H}(\mathbf{x}_{n-1} - \mathbf{x}_n) e^{-i\mathbf{k}_q \cdot (\mathbf{x}_{n-1} - \mathbf{x}_n)} \\
&\quad \times S_n^{(p)}(\mathbf{x}_1, \mathbf{x}_2, \dots, \mathbf{x}_n), \quad \text{for } n \geq 2. \tag{S82}
\end{aligned}$$

An explicit expression for the nonlocal strong-contrast expansions is obtained by substituting Eq. (S81) into Eq. (S80) and by following the calculations analogous to Eqs. (S71) and (S72):

$$\begin{aligned}
&(\phi_p \beta_{pq})^2 \left[ \frac{\varepsilon_e(\mathbf{k}_q) - \varepsilon_q \mathbf{I}}{\varepsilon_e(\mathbf{k}_q) + (d-1)\varepsilon_q \mathbf{I}} \right]^{-1} \\
&= \frac{(\phi_p d\varepsilon_q \beta_{pq})^2}{d\varepsilon_q} (\phi_p d\varepsilon_q \beta_{pq})^{-1} \left\{ \mathbf{I} - \left[ \mathbb{A}_2 + \mathbb{A}_3 + \dots \right] (\phi_p d\varepsilon_q \beta_{pq})^{-1} + \left[ \mathbb{A}_2 + \mathbb{A}_3 + \dots \right]^2 (\phi_p d\varepsilon_q \beta_{pq})^{-2} \right. \\
&\quad \left. - \left[ \mathbb{A}_2 + \mathbb{A}_3 + \dots \right]^3 (\phi_p d\varepsilon_q \beta_{pq})^{-3} + \dots \right\} + \frac{(\phi_p d\varepsilon_q \beta_{pq})^2}{d\varepsilon_q} \int_{\epsilon} d\mathbf{x}_1 \mathbf{H}(\mathbf{x}_1) e^{-i\mathbf{k}_q \cdot \mathbf{x}_1} \\
&= \phi_p \beta_{pq} \mathbf{I} - \frac{1}{d\varepsilon_q} \left[ \mathbb{A}_2 - (d\varepsilon_q \beta_{pq})^2 \phi_p^2 \int_{\epsilon} d\mathbf{r}_1 \mathbf{H}(\mathbf{r}_1) e^{-i\mathbf{k}_q \cdot \mathbf{r}_1} \right] - \frac{1}{d\varepsilon_q} \left[ \mathbb{A}_3 - \mathbb{A}_2 \mathbb{A}_2 (\phi_p d\varepsilon_q \beta_{pq})^{-1} \right] \\
&\quad - \frac{1}{d\varepsilon_q} \left[ \mathbb{A}_4 - \left( \mathbb{A}_2 \mathbb{A}_3 + \mathbb{A}_3 \mathbb{A}_2 \right) (\phi_p d\varepsilon_q \beta_{pq})^{-1} + \mathbb{A}_2 \mathbb{A}_2 \mathbb{A}_2 (\phi_p d\varepsilon_q \beta_{pq})^{-2} \right] + \dots \tag{S83}
\end{aligned}$$

Substituting the definitions of  $\bigcirc \mathbb{A}_n$  given in Eq. (S82) into the above expression leads to

$$\begin{aligned}
(\phi_p \beta_{pq})^2 \left[ \frac{\varepsilon_e(\mathbf{k}_q) - \varepsilon_q \mathbf{I}}{\varepsilon_e(\mathbf{k}_q) + (d-1)\varepsilon_q \mathbf{I}} \right]^{-1} &= \phi_p \beta_{pq} \mathbf{I} - d\varepsilon_q \beta_{pq}^2 \int_{\epsilon} d\mathbf{x}_1 \mathbf{H}(\mathbf{x}_1 - \mathbf{x}_2) e^{-i\mathbf{k}_q \cdot (\mathbf{x}_1 - \mathbf{x}_2)} \chi_V(\mathbf{x}_1 - \mathbf{x}_2) \\
&- \frac{(d\varepsilon_q \beta_{pq})^3}{\phi_p d\varepsilon_q} \int_{\epsilon} d\mathbf{x}_1 d\mathbf{x}_2 \mathbf{H}(\mathbf{x}_1 - \mathbf{x}_2) e^{-i\mathbf{k}_q \cdot (\mathbf{x}_1 - \mathbf{x}_2)} \cdot \mathbf{H}(\mathbf{x}_2 - \mathbf{x}_3) e^{-i\mathbf{k}_q \cdot (\mathbf{x}_2 - \mathbf{x}_3)} \\
&\times \left[ \phi_p S_3^{(p)}(\mathbf{x}_1, \mathbf{x}_2, \mathbf{x}_3) - S_2^{(p)}(\mathbf{x}_1, \mathbf{x}_2) S_2^{(p)}(\mathbf{x}_2, \mathbf{x}_3) \right] \\
&- \frac{(d\varepsilon_q \beta_{pq})^4}{\phi_p^2 d\varepsilon_q} \int_{\epsilon} d\mathbf{x}_1 d\mathbf{x}_2 \mathbf{H}(\mathbf{x}_1 - \mathbf{x}_2) e^{-i\mathbf{k}_q \cdot (\mathbf{x}_1 - \mathbf{x}_2)} \cdot \mathbf{H}(\mathbf{x}_2 - \mathbf{x}_3) e^{-i\mathbf{k}_q \cdot (\mathbf{x}_2 - \mathbf{x}_3)} \cdot \mathbf{H}(\mathbf{x}_3 - \mathbf{x}_4) e^{-i\mathbf{k}_q \cdot (\mathbf{x}_3 - \mathbf{x}_4)} \\
&\times \left[ \phi_p^2 S_4^{(p)}(\mathbf{x}_1, \mathbf{x}_2, \mathbf{x}_3, \mathbf{x}_4) - \phi_p S_2^{(p)}(\mathbf{x}_1, \mathbf{x}_2) S_3^{(p)}(\mathbf{x}_2, \mathbf{x}_3, \mathbf{x}_4) - \phi_p S_3^{(p)}(\mathbf{x}_1, \mathbf{x}_2, \mathbf{x}_3) S_2^{(p)}(\mathbf{x}_3, \mathbf{x}_4) \right. \\
&\left. + S_2^{(p)}(\mathbf{x}_1, \mathbf{x}_2) S_2^{(p)}(\mathbf{x}_2, \mathbf{x}_3) S_2^{(p)}(\mathbf{x}_3, \mathbf{x}_4) \right] + \dots
\end{aligned} \tag{S84}$$

$$= \phi_p \beta_{pq} \mathbf{I} - \sum_{n=2}^{\infty} \mathbf{A}_n^{(p)}(\mathbf{k}_q) \beta_{pq}^n, \tag{S85}$$

where the  $n$ th order coefficient  $\mathbf{A}_n^{(p)}(\mathbf{k}_q)$  is defined as

$$\mathbf{A}_2^{(p)}(\mathbf{k}_q) = d\varepsilon_q \int_{\epsilon} \mathbf{H}^{(q)}(\mathbf{r}) e^{-i\mathbf{k}_q \cdot \mathbf{r}} \chi_V(\mathbf{r}) d\mathbf{r}, \tag{S86}$$

$$\begin{aligned}
\mathbf{A}_n^{(p)}(\mathbf{k}_q) &= d\varepsilon_q \left( \frac{-d\varepsilon_q}{\phi_p} \right)^{n-2} \int_{\epsilon} \mathbf{H}^{(q)}(\mathbf{x}_1 - \mathbf{x}_2) e^{-i\mathbf{k}_q \cdot (\mathbf{x}_1 - \mathbf{x}_2)} \dots \mathbf{H}^{(q)}(\mathbf{x}_{n-1} - \mathbf{x}_n) e^{-i\mathbf{k}_q \cdot (\mathbf{x}_{n-1} - \mathbf{x}_n)} \\
&\times \Delta_n^{(p)}(\mathbf{x}_1, \dots, \mathbf{x}_n) d\mathbf{x}_1 \dots d\mathbf{x}_{n-1}, \quad n \geq 3,
\end{aligned} \tag{S87}$$

and  $\Delta_n^{(p)}(\mathbf{x}_1, \dots, \mathbf{x}_n)$  is given in Eq. (59) in the main text.

### III. PROPERTIES OF NONLOCAL ATTENUATION FUNCTION $F(Q)$

For macroscopically isotropic media in  $\mathbb{R}^d$ , *nonlocal attenuation function*  $F(\mathbf{Q})$  is the key microstructure-dependent parameter in the strong-contrast approximation, which is related to the second-rank tensor  $\mathbf{A}_2^{(p)}(\mathbf{k}_q)$  given in Eq. (S86):

$$\mathbf{A}_2^{(p)}(\mathbf{k}_q) \equiv \frac{1}{d} \text{Tr}[\mathbf{A}_2^{(p)}(\mathbf{k}_q)] = -\frac{(d-1)\pi}{2^{d/2} \Gamma(d/2)} F(\mathbf{k}_q). \tag{S88}$$

For a statistically anisotropic two-phase medium, the nonlocal attenuation function is explicitly written as

$$F(\mathbf{Q}) \equiv -\frac{2^{d/2} \Gamma(d/2)}{\pi} Q^2 \int \frac{i}{4} \left( \frac{Q}{2\pi r} \right)^{d/2-1} \mathcal{H}_{d/2-1}^{(1)}(Qr) e^{-i\mathbf{Q} \cdot \mathbf{r}} \chi_V(\mathbf{r}) d\mathbf{r} \tag{S89}$$

$$= -\frac{\Gamma(d/2)}{2^{d/2} \pi^{d+1}} Q^2 \int \frac{\tilde{\chi}_V(\mathbf{q})}{|\mathbf{q} + \mathbf{Q}|^2 - Q^2} d\mathbf{q}. \tag{S90}$$

Note that (S90) is the Fourier representation of Eq. (S89), which can be immediately obtained from the Parseval theorem by utilizing the fact that  $1/[q^2 - Q^2]$  is the radial Fourier transform of  $(i/4)[Q/(2\pi r)]^{d/2-1} \mathcal{H}_{d/2-1}^{(1)}(Qr)$ .

For statistically isotropic media, the nonlocal attenuation function depends on wavenumber  $Q$ , instead of wavevector  $\mathbf{Q}$ . Its imaginary and real parts can be simplified as

$$\text{Im}[F(Q)] = \begin{cases} -\frac{Q^2}{\pi^2} \int_0^{\pi/2} \tilde{\chi}_V(2Q \cos \phi) d\phi, & d = 2 \\ -\frac{Q}{2(2\pi)^{3/2}} \int_0^{2Q} q \tilde{\chi}_V(q) dq, & d = 3 \end{cases} \tag{S91}$$

$$\text{Re}[F(Q)] = -\frac{2Q^2}{\pi} \text{p.v.} \int_0^{\infty} dq \frac{1}{q(Q^2 - q^2)} \text{Im}[F(q)], \tag{S92}$$

respectively, where Eq. (S92) is valid for  $d = 2, 3$ .

In this section, we derive and present some important properties of the nonlocal attenuation function. We first derive  $F(\mathbf{Q})$  for hypercubic lattice packings that are macroscopically isotropic but statistically anisotropic in Sec. III A. We then investigate some general properties of  $F(Q)$  for statistically isotropic media. Specifically, in Sec. III B–III D, we derive some of its analytic properties, its alternative formulas [Eqs. (S91) and (S92)], and its asymptotic expressions, respectively.

### A. Formulas for Hypercubic Lattice Packings

For a hypercubic lattice ( $\mathbb{Z}^d$ ) packing in  $\mathbb{R}^d$ , its effective dielectric constant tensor possesses the cubic symmetry but has  $\mathbf{k}_q$ -dependence because  $\mathbb{Z}^d$  is statistically anisotropic, i.e.,  $\varepsilon_e(\mathbf{k}_q) = \varepsilon_e(\mathbf{k}_q) \mathbf{I}$ . In this section, we derive the analytic expression of  $\varepsilon_e(\mathbf{k}_q)$  for  $\mathbb{Z}^d$  packings ( $d = 2, 3$ ) using the general definition (S90) of the attenuation function. For concreteness, we take the matrix and reference phases as phase 1, and the particle phase as phase 2.

We first obtain the attenuation function of  $\mathbb{Z}^d$  sphere packings. For a  $\mathbb{Z}^d$  sphere packing of packing fraction  $\phi_2$  and lattice constant  $L$ , its spectral density is written as

$$\tilde{\chi}_v(\mathbf{Q}) = \rho \tilde{m}(Q; a)^2 S(\mathbf{Q}) = (2\pi)^d \rho^2 \tilde{m}(Q; a)^2 \sum_{\mathbf{G} \in \mathbb{Z}^{d*} \setminus \mathbf{0}} \delta(\mathbf{Q} - \mathbf{G}/L), \quad (\text{S93})$$

where  $\rho = L^{-d}$  is number density,  $a$  is particle radius,  $Q \equiv |\mathbf{Q}|$ ,  $\mathbb{Z}^{d*}$  is the reciprocal lattice of the unit  $\mathbb{Z}^d$  lattice,  $\tilde{m}(Q; a) = (2\pi a/Q)^{d/2} J_{d/2}(Qa)$ , and  $S(\mathbf{Q})$  is the structure factor of a hypercubic lattice. Applying Eq. (S93) to Eq. (S90) yields

$$F(\mathbf{Q}) = - \frac{2^{d/2} \Gamma(d/2)}{\pi} \rho^2 (QL)^2 \sum_{\mathbf{G} \in \mathbb{Z}^{d*} \setminus \mathbf{0}} \frac{\tilde{m}(|\mathbf{G}|/L; a)^2}{\mathbf{G} \cdot (\mathbf{G} + 2\mathbf{Q}L)}, \quad (\text{S94})$$

if the Laue condition of  $L\mathbb{Z}^d$  lattice is unmet [i.e.,  $\mathbf{G} \cdot (\mathbf{G} + 2\mathbf{Q}L) \neq 0$ ]. Here,  $\mathbb{Z}^{d*}$  stands for the reciprocal lattice of  $\mathbb{Z}^d$ . Note that Eq. (S94) is real-valued.

Using Eq. (S94), we obtain two-point approximation of  $\varepsilon_e(\mathbf{k}_1)$  for a hypercubic lattice packing:

$$\frac{\varepsilon_e(\mathbf{k}_1)}{\varepsilon_1} = 1 + d\phi_2^2 \beta_{21} \left[ \phi_2(1 - \phi_2 \beta_{21}) + (d-1)(\rho k_1 L)^2 \beta_{21} \sum_{\mathbf{G} \in \mathbb{Z}^{d*} \setminus \mathbf{0}} \frac{\tilde{m}(|\mathbf{G}|/L; a)^2}{\mathbf{G} \cdot (\mathbf{G} + 2\mathbf{k}_1 L)} \right]^{-1}, \quad (\text{S95})$$

where  $\beta_{21}$  is defined in Eq. (S2). We use Eq. (S95) with  $\mathbf{k}_1 = k_1 \hat{\mathbf{x}}$  to estimate  $\varepsilon_e$  of periodic packings along the  $\Gamma$ - $X$  direction (see Sec. VIII of the main text).

### B. Analytic Properties

We now show that  $F(Q)$  has the following analytic properties for statistically isotropic media in  $\mathbb{R}^d$ :

1.  $F(Q)$  is an analytic function of a complex variable  $Q$  in the *upper half-plane*, i.e.,  $\text{Im}[Q] \geq 0$ ;
2.  $\text{Re}[F(Q)]$  and  $\text{Im}[F(Q)]$  are even and odd functions of real variable  $Q$ , respectively.

To do so, we start by rewriting Eq. (S89) as follows:

$$\begin{aligned} F(Q) &= -i 2^{(d-2)/2} \Gamma(d/2) Q^2 \int_0^\infty r \mathcal{H}_{d/2-1}^{(1)}(Qr) J_{d/2-1}(Qr) \chi_v(r) dr \\ &= -i 2^{(d-2)/2} \Gamma(d/2) \int_0^{\text{sgn}(Q)\infty} x \mathcal{H}_{d/2-1}^{(1)}(x) J_{d/2-1}(x) \chi_v(x/Q) dx, \end{aligned} \quad (\text{S96})$$

where  $\text{sgn}(Q)$  is the sign of a real number  $Q$ , and we have used the formula for the radial Fourier transform in  $\mathbb{R}^d$

$$\tilde{f}(Q) = \int f(r) e^{-i\mathbf{Q} \cdot \mathbf{r}} d\mathbf{r} = (2\pi)^{d/2} \int_0^\infty r^{d-1} f(r) \frac{J_{(d-2)/2}(Qr)}{(Qr)^{(d-2)/2}} dr.$$

Property 1 follows from the observation that, if Eq. (S96) is regarded as a function in the complex  $Q$  plane, this integral is well-defined for  $\text{Im}[Q] \geq 0$  because as  $|x|$  increases at a constant angle  $\arg x$  (or, equivalently, as  $r$  goes to infinity with  $Q$  fixed),

$$x \mathcal{H}_{d/2-1}^{(1)}(x) J_{d/2-1}(x) \sim \begin{cases} \frac{1}{\pi} e^{2i[x-(d-1)\pi/4]}, & -\pi < \arg x < 0 \\ \frac{1}{\pi}, & 0 < \arg x < \pi \end{cases}, \quad \text{as } |x| \rightarrow \infty.$$

Property 2 immediately follows from the fact that the real and imaginary parts of  $ix \mathcal{H}_{d/2-1}^{(1)}(x) J_{d/2-1}(x)$  are even and odd function of  $x$ , respectively, for  $d = 2, 3$ .

### C. Alternative Formulas

In this subsection, we derive Eqs. (S91) and (S92) from a general Fourier-space representation of  $F(\mathbf{Q})$  given in Eq. (S90). In three dimensions, without loss of generality, we can take  $\mathbf{Q} = Q\hat{\mathbf{z}}$ . We write Eq. (S90) in spherical coordinates:

$$\begin{aligned} \int d\mathbf{q} \frac{\tilde{\chi}_v(\mathbf{q})}{|\mathbf{q} + Q\hat{\mathbf{z}}|^2 - Q^2} &= \int_0^\infty dq q^2 \int_0^\pi d\theta \sin \theta \left[ \int_0^{2\pi} d\phi \right] \frac{\tilde{\chi}_v(q)}{q(q + 2Q \cos \theta)} \\ &= 2\pi \int_{-1}^1 dx \int_0^\infty dq \frac{q \tilde{\chi}_v(q)}{q + 2Qx} \end{aligned} \quad (\text{S97})$$

$$\begin{aligned} &= \pi \left[ \int_{-1}^1 dx \int_0^\infty dq \frac{q \tilde{\chi}_v(q)}{q + 2Qx} + \int_1^{-1} (-1) dx' \int_0^\infty dq' (-1) \frac{-q' \tilde{\chi}_v(-q')}{-q' - 2Qx'} \right] \\ &= \pi \int_{-1}^1 dx \int_{-\infty}^\infty dq \frac{q \tilde{\chi}_v(q)}{q + 2Qx}, \end{aligned} \quad (\text{S98})$$

where we use  $\tilde{\chi}_v(q) = \tilde{\chi}_v(-q)$  to obtain Eq. (S98). Since  $F(Q)$  is analytic for  $\text{Im}[Q] \geq 0$  (see Sec. IIIB), applying the following identity

$$\int_{-\infty}^\infty dx \frac{f(x)}{x - x'} = \lim_{\epsilon \rightarrow 0^+} \int_{-\infty}^\infty dx \frac{f(x)}{x - (x' \pm i\epsilon)} = \text{p.v.} \int_{-\infty}^\infty dx \frac{f(x)}{x - x'} \pm i\pi f(x') \quad (\text{S99})$$

to Eq. (S98) yields

$$\begin{aligned} F(Q) &= -\frac{Q^2}{(2\pi)^{5/2}} \int_{-1}^1 dx \int_{-\infty}^\infty dq \frac{q \tilde{\chi}_v(q)}{q + 2x(Q + i\epsilon)} \\ &= -\frac{Q^2}{(2\pi)^{5/2}} \int_{-1}^1 dx \left[ \text{p.v.} \int_{-\infty}^\infty dq \frac{q \tilde{\chi}_v(q)}{q + 2xQ} + i\pi \text{sgn}(x) (2Qx) \tilde{\chi}_v(2Qx) \right] \\ &= -\frac{Q^2}{(2\pi)^{5/2}} \int_{-1}^1 dx \left[ \text{p.v.} \int_{-\infty}^\infty dq \frac{q \tilde{\chi}_v(q)}{q + 2xQ} + i\pi 2Q|x| \tilde{\chi}_v(2Qx) \right] \\ &= -\frac{4Q^2}{(2\pi)^{5/2}} \int_0^1 dx \left[ \text{p.v.} \int_0^\infty dq \frac{q^2 \tilde{\chi}_v(q)}{q^2 - (2xQ)^2} \right] - \frac{iQ}{2(2\pi)^{3/2}} \int_0^{2Q} dq' q' \tilde{\chi}_v(q'), \end{aligned} \quad (\text{S100})$$

where p.v. stands for the Cauchy principal value of an improper integral. Since each integral in Eq. (S100) is real-valued, the real and imaginary parts of  $F(Q)$  can be written as

$$\text{Re}[F(Q)] = -\frac{4Q^2}{(2\pi)^{5/2}} \int_0^1 dx \left[ \text{p.v.} \int_0^\infty dq \frac{q^2 \tilde{\chi}_v(q)}{q^2 - (2xQ)^2} \right], \quad (\text{S101})$$

$$\text{Im}[F(Q)] = -\frac{Q}{2(2\pi)^{3/2}} \int_0^{2Q} dq q \tilde{\chi}_v(q), \quad (\text{S102})$$

respectively.

When computing  $F(Q)$  from the isotropic spectral density obtained from experiments or numerical simulations, it is easy to compute the imaginary part given in Eq. (S102) but difficult to compute the real part (S101). For this

reason, we derive an alternative formula for the real part [Eq. (S101)]. We first interchange the order of integrals in Eq. (S101), change variables such that  $q \rightarrow 2q'x$  and  $x \rightarrow q''/(2q')$ , and replace the integral over  $q''$  with Eq. (S102) to obtain

$$\begin{aligned} \text{Re}[F(Q)] &= -\frac{4Q^2}{(2\pi)^{5/2}} \text{p.v.} \int_0^\infty dq \int_0^1 dx \frac{q^2 \tilde{\chi}_v(q)}{q^2 - (2Qx)^2} \\ &= -\frac{2Q^2}{(2\pi)^{5/2}} \text{p.v.} \int_0^\infty dq' \frac{1}{q'^2 - Q^2} \int_0^{2q'} dq'' q'' \tilde{\chi}_v(q'') \\ &= -\frac{2Q^2}{\pi} \text{p.v.} \int_0^\infty dq \frac{\text{Im}[F(q)]}{q(Q^2 - q^2)}. \end{aligned} \quad (\text{S103})$$

Thus, we have derived Eqs. (S91) and (S92) for three dimensions.

In two dimensions, we rewrite the integral in Eq. (S90) in cylindrical coordinates:

$$\begin{aligned} \int d\mathbf{q} \frac{\tilde{\chi}_v(\mathbf{q})}{|\mathbf{q} + Q\hat{\mathbf{x}}|^2 - Q^2} &= \int_0^{2\pi} d\phi \int_0^\infty dq \frac{\tilde{\chi}_v(q)}{q + 2Q \cos \phi} \\ &= 2 \int_0^\pi d\phi \int_0^\infty dq \frac{\tilde{\chi}_v(q)}{q + 2Q \cos \phi} = 2 \int_0^{\pi/2} d\phi \int_0^\infty dq \left[ \frac{1}{q + 2Q \cos \phi} + \frac{1}{q - 2Q \cos \phi} \right] \tilde{\chi}_v(q) \\ &= 2 \int_0^{\pi/2} d\phi \int_{-\infty}^\infty dq \left[ \frac{1}{q + 2(Q + i\epsilon) \cos \phi} + \frac{1}{q - 2(Q + i\epsilon) \cos \phi} \right] \Theta(q) \tilde{\chi}_v(q), \end{aligned} \quad (\text{S104})$$

where  $\epsilon$  is an infinitesimal positive number, and  $\Theta(x) \equiv \begin{cases} 1, & x > 0 \\ 0, & \text{otherwise} \end{cases}$  is Heaviside step function. Applying the identity (S99) to the integral over  $q$  in Eq. (S104) gives

$$\begin{aligned} &\int_{-\infty}^\infty dq \left[ \frac{1}{q + 2(Q + i\epsilon) \cos \phi} + \frac{1}{q - 2(Q + i\epsilon) \cos \phi} \right] \Theta(q) \tilde{\chi}_v(q) \\ &= \text{p.v.} \int_0^\infty dq \frac{2q \tilde{\chi}_v(q)}{q^2 - (2Q \cos \phi)^2} + i\pi \tilde{\chi}_v(2Q \cos \phi). \end{aligned} \quad (\text{S105})$$

Combining Eq. (S105) to Eqs. (S104) and (S90), we obtain

$$\text{Re}[F(Q)] = -\frac{Q^2}{\pi^3} \int_0^{\pi/2} d\phi \left[ \text{p.v.} \int_0^\infty dq \frac{2q \tilde{\chi}_v(q)}{q^2 - (2Q \cos \phi)^2} \right], \quad (\text{S106})$$

$$\text{Im}[F(Q)] = -\frac{Q^2}{\pi^2} \int_0^{\pi/2} d\phi \tilde{\chi}_v(2Q \cos \phi). \quad (\text{S107})$$

As we done in three dimensions, we derive an alternative expression for Eq. (S106). We first interchange the order of integrals, change variables of integration  $q \rightarrow 2q' \cos \phi$ , and then substitute the integral over  $\phi$  with Eq. (S107):

$$\text{Re}[F(Q)] = -\frac{Q^2}{\pi^3} \text{p.v.} \int_0^\infty dq \int_0^{\pi/2} d\phi \frac{2q \tilde{\chi}_v(q)}{q^2 - (2Q \cos \phi)^2} \quad (\text{S108})$$

$$= -\frac{2Q^2}{\pi^3} \text{p.v.} \int_0^\infty dq' \frac{q'}{q'^2 - Q^2} \int_0^{\pi/2} d\phi \tilde{\chi}_v(2q' \cos \phi) \quad (\text{S109})$$

$$= -\frac{2Q^2}{\pi} \text{p.v.} \int_0^\infty dq \frac{\text{Im}[F(q)]}{q(Q^2 - q^2)}. \quad (\text{S110})$$

Thus, we have derived Eqs. (S91) and (S92) for two dimensions.

#### Remarks:

1. Similar to the Kramers-Kronig relations, the expression (S92) is in fact a natural consequence of the analytic properties of  $F(Q)$ .

2. In practice, it is nontrivial to numerically compute the Cauchy principal value in Eq. (S92). To avoid such problems, we change this integral into a more numerically tractable form by utilizing the fact that  $\text{Im}[F(Q)] \sim Q$  as  $Q \rightarrow \infty$  (see Sec. IIID):

$$\begin{aligned} \text{Re}[F(Q)] &\approx -\frac{2Q^2}{\pi} \left[ \text{p.v.} \int_0^M \frac{1}{q(Q^2 - q^2)} \text{Im}[F(q)] dq + \frac{\text{Im}[F(M)]}{M} \int_M^\infty \frac{1}{Q^2 - q^2} dq \right] \\ &= -\frac{2Q}{\pi} \left( \int_0^M \frac{\text{Im}[F(q)]}{(Q+q)q} dq + \int_0^M \frac{\text{Im}[F(q)] - \text{Im}[F(Q)]}{Q^2 - q^2} dq \right. \\ &\quad \left. + \frac{1}{2Q} \left\{ \text{Im}[F(Q)] - \frac{Q}{M} \text{Im}[F(M)] \right\} \ln \left| \frac{M+Q}{M-Q} \right| \right), \end{aligned} \quad (\text{S111})$$

where  $M$  is an upper limit of the integral.

#### D. Asymptotic Behaviors

In this subsection, we derive general asymptotic expressions for  $F(Q)$  in the quasistatic (small- $Q$ ) and large- $Q$  regimes. The reader is referred to Eqs. (83) and (84) in the main text for the small- $Q$  behaviors of  $\text{Im}[F(Q)]$  and  $\text{Re}[F(Q)]$ , respectively. The large- $Q$  asymptotic behaviors are

$$\text{Im}[F(Q)] \sim Q + \mathcal{O}(Q^{-1}), \quad (\text{S112})$$

$$\text{Re}[F(Q)] \sim \text{const.}(< 0), \quad (\text{S113})$$

regardless of the functional form of the spectral density.

The small- $Q$  expressions are easy to derive. For Eq. (84) in the main text, it can be derived from Eq. (S96):

$$\begin{aligned} \text{Re}[F(Q)] &= 2^{(d-2)/2} \Gamma(d/2) Q^2 \int_0^\infty r Y_{d/2-1}(Qr) J_{d/2-1}(Qr) \chi_V(r) dr \\ &= 2^{(d-2)/2} \Gamma(d/2) Q^2 \int_0^\infty \left[ -\frac{r \Gamma(d/2-1)}{\pi \Gamma(d/2)} + \mathcal{O}(Q^{d-2} r^{d-1}) \right] \chi_V(r) dr \\ &\sim -Q^2 \int_0^\infty r \chi_V(r) dr \sim -Q^2, \text{ as } Q \rightarrow 0^+. \end{aligned}$$

The small- $Q$  behavior of  $\text{Im}[\varepsilon_e(Q)]$ , given in Eq. (83) in the main text, can be easily derived from Eq. (S91).

The large- $Q$  behaviors are slightly more complicated to derive. To show Eq. (S112), we note that  $\text{Im}[F(Q)]/Q$  given in Eq. (S91) is identical to the integral of  $\tilde{\chi}_V(q)$  on a  $d$ -dimensional spherical surface of radius  $Q$  centered at  $\mathbf{q} = Q\hat{\mathbf{x}}$  up to a proportional constant. Furthermore, for any  $Q > 0$ , this integral is bounded above by the volume integral of a non-negative function  $\tilde{\chi}_V(q)$  that converges to a finite value  $(2\pi)^d \chi_V(0)$ , i.e.,

$$\left| \frac{\text{Im}[F(Q)]}{Q} \right| \propto \int_{|\mathbf{q}-Q\hat{\mathbf{x}}|=Q} d\mathbf{q} \tilde{\chi}_V(q) < \int_{\mathbb{R}^d} d\mathbf{q} \tilde{\chi}_V(q) = (2\pi)^d \chi_V(0).$$

These two observations lead us to conclude that  $\text{Im}[F(Q)]/Q$  converges to a negative constant as  $Q$  goes to infinity, which is identical to Eq. (S112). A simple asymptotic analysis of Eqs. (S92) and (S112) yields Eq. (S113).

#### IV. COMPARISONS OF LOCAL AND NONLOCAL ATTENUATION FUNCTIONS

Here we compare the behaviors of the “local” attenuation function  $\mathcal{F}(Q)$  derived in Ref. 1 for the quasistatic strong-contrast to its nonlocal counterpart  $F(\mathbf{Q})$  [cf. (S89) or (S90)] derived in the present work. Both the local and nonlocal attenuation functions depend on the spectral density, but their functional behaviors are generally different across wavenumbers. We also provide plots of both the real and imaginary parts of the nonlocal attenuation function  $F(\mathbf{Q})$  for the four models of disordered two-phase media considered in this work.

The local attenuation  $\mathcal{F}(Q)$  is defined in Eqs. (S7) and (S8). In contrast to the nonlocal attenuation function  $F(\mathbf{Q})$ , the local attenuation function only depends on the wavenumber  $Q$ , instead of the wavevector  $\mathbf{Q}$ . For statistically isotropic media, its real and imaginary parts are given in Eqs. (S15) and (S13), respectively.

As expected, the local and nonlocal attenuation functions,  $\mathcal{F}(Q)$  and  $F(Q)$ , are identical in the quasistatic (small- $Q$ ) regime. Specifically, the small- $Q$  behaviors of  $\text{Im}[\mathcal{F}(Q)]$  and  $\text{Im}[F(Q)]$  are given in Eq. (S18) and Eq. (83) in the main text. The small- $Q$  behaviors of  $\text{Re}[\mathcal{F}(Q)]$  and  $\text{Re}[F(Q)]$  are given in Eq. (S19) and Eq. (84) in the main text. Beyond the quasistatic regime, however, both types of attenuation functions become increasingly different as the wavenumber  $k_q$  increases, with concomitant distinctly different attenuation characteristics. In the large- $Q$  regime, the local and nonlocal attenuation functions exhibit considerably different behaviors:

$$\text{Im}[\mathcal{F}(Q)] \sim Q^{-1}, \quad \text{Re}[\mathcal{F}(Q)] \rightarrow \frac{2^{d/2} \Gamma(d/2)}{\pi} \phi_p (1 - \phi_p) \quad (> 0), \quad \text{as } Q \rightarrow \infty \quad (\text{S114})$$

$$\text{Im}[F(Q)] \sim Q, \quad \text{Re}[F(Q)] \rightarrow \text{const.} \quad (< 0), \quad \text{as } Q \rightarrow \infty. \quad (\text{S115})$$

The reader is referred to Secs. IB and III for derivations.

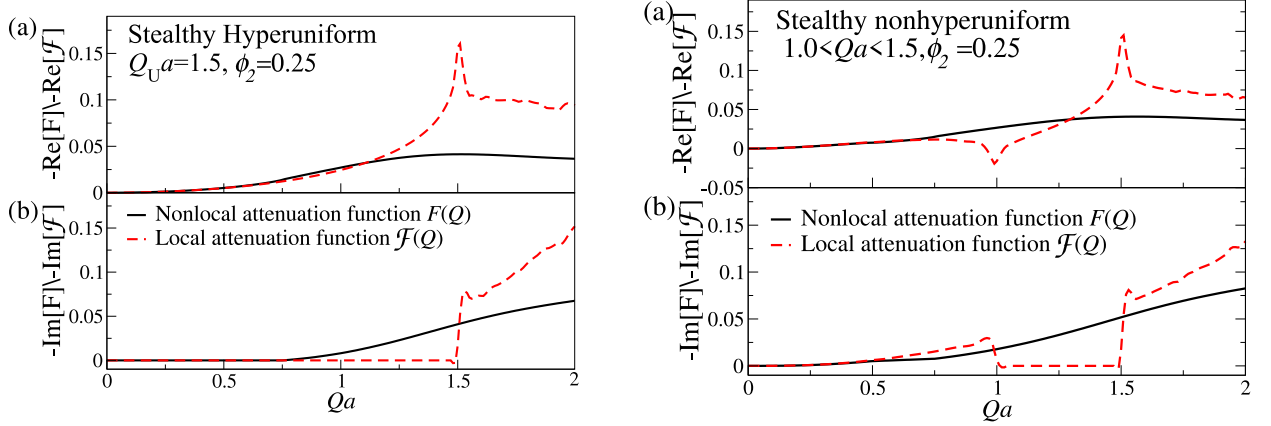

FIG. S2. Comparison of negatives of (a) the real and (b) imaginary parts of the nonlocal attenuation function  $F(Q)$  [see Eq. (S96)] and its local counterpart  $\mathcal{F}(Q)$  [see Eq. (S7)] as functions of dimensionless wavenumber  $Qa$  for 3D disordered models. We consider (left panel) stealthy hyperuniform packings and (right panel) stealthy nonhyperuniform packings of packing fraction  $\phi_2 = 0.25$  and identical spheres of radius  $a$ .

We compare both attenuation functions  $\mathcal{F}(Q)$  and  $F(Q)$  for stealthy hyperuniform packings; see Fig. S2 for 3D cases. While these two functions are identical in the quasistatic regime, they become increasingly different from one another as the wavenumber increases. For example, Eqs. (S91) and (S13) immediately show that for stealthy hyperuniform systems [i.e.,  $\tilde{\chi}_v(Q) = 0$  for  $Q < Q_U$ ], the imaginary parts of these two attenuation functions are identically zero (transparent or lossless) up to finite but quite different range of wavenumbers; specifically,

$$\begin{cases} \text{Im}[F(Q)] = 0, & \text{where } Q < Q_U/2, \\ \text{Im}[\mathcal{F}(Q)] = 0, & \text{where } Q < Q_U. \end{cases} \quad (\text{S116})$$

We also present a plot comparing both local and nonlocal attenuation functions [Eqs. (S7) and (S96), respectively] for stealthy nonhyperuniform dispersions [i.e.,  $\tilde{\chi}_v(Q) = 0$  for  $0 < Q_L < Q < Q_U$ ]. Specifically, we consider three-dimensional stealthy nonhyperuniform sphere packings of radius  $a$  and packing fraction  $\phi_2 = 0.25$ , and they are stealthy in the region of  $1.0 < Qa < 1.5$ . As shown in Fig. S2, both attenuation functions are identical only in the quasistatic regime, as observed in the stealthy hyperuniform packings. Beyond that regime, importantly, the local attenuation incorrectly predicts that these media are transparent for  $1 < k_q a < 1.5$ , the nonlocal attenuation function successfully captures the fact that they are not transparent.

## V. KRAMERS-KRONIG RELATIONS

Here, we elaborate on some details about the Kramers-Kronig relations that are omitted in the main text for brevity. We focus on the “unmodified” strong-contrast approximation because it has the same behavior as the scaled variant. We define a complex function  $f(k_q) \equiv \varepsilon_e(k_q) - \varepsilon_q$ , which is equal to  $[a + b F(k_q)]^{-1}$  for the strong-contrast approximation, where  $a$  and  $b$  are constant real numbers. The following three properties of  $F(k_q)$  [ $F(k_q)$  is an analytic function in the upper half-plane of complex variable  $k_q$ ;  $F(k_q)$  diverges like  $|k_q|$  as  $|k_q|$  goes to infinity;  $\text{Re}[F(k_q)]$  and  $\text{Im}[F(k_q)]$  are even and odd functions of  $k_q$ , respectively], shown in Secs. III and III D, lead  $f(k_q)$  to possess the following three properties:

- (i)  $\varepsilon_e(k_q)$  is an analytic function in the *upper half-plane* of  $k_q$ ;
- (ii)  $f(k_q) = \varepsilon(k_q) - \varepsilon_q$  vanishes like  $1/|k_q|$  as  $|k_q|$  goes to infinity; and
- (iii)  $\text{Re}[f(k_q)]$  and  $\text{Im}[f(k_q)]$  are even and odd functions of  $k_q$ , respectively.

Note that any complex function  $f(q)$  exhibiting properties (i) and (ii) satisfies the following relations, which correspond to the Kramer-Kronig relations in general context:

$$\begin{aligned}\text{Re}[f(k_q)] &= \frac{1}{\pi} \text{p.v.} \int_{-\infty}^{\infty} dq \frac{\text{Im}[f(q)]}{k_q - q} \\ \text{Im}[f(k_q)] &= -\frac{1}{\pi} \text{p.v.} \int_{-\infty}^{\infty} dq \frac{\text{Re}[f(q)]}{k_q - q}.\end{aligned}$$

By combining these relations with the property (iii) of  $f(k_q)$ , one can immediately show that the strong-contrast approximations (both unmodified and scaled ones) meet the Kramer-Kronig relations given in the main text:

$$\text{Re}[\varepsilon_e(k_q)] = \varepsilon_q + \frac{2}{\pi} \text{p.v.} \int_0^{\infty} dq \frac{q \text{Im}[\varepsilon_e(q)]}{q^2 - k_q^2}, \quad (\text{S117})$$

$$\text{Im}[\varepsilon_e(k_q)] = -\frac{2k_q}{\pi} \text{p.v.} \int_0^{\infty} dq \frac{\text{Re}[\varepsilon_e(q)] - \varepsilon_q}{q^2 - k_q^2}. \quad (\text{S118})$$

This result makes sense because the strong-contrast approximations or, equivalently, the nonlocal attenuation function  $F(Q)$  come from  $\mathbf{G}^{(q)}(\mathbf{x}, \mathbf{x}')$  given in Eq. (S30) that is the temporal Fourier transform of the *retarded* Green function  $\mathbf{G}^{(q)}(\mathbf{x}, t, \mathbf{x}', t')$  [4] accounting for causality.

For illustrative purpose, we compare the effective dielectric constant  $\varepsilon_e(k_q)$  from the strong-contrast approximation with its transformation via the Kramers-Kronig relations. We consider 3D equilibrium packings of packing fraction  $\phi_2 = 0.25$  and contrast ratio  $\varepsilon_2/\varepsilon_1 = 4$ ; see Fig. S3. Specifically, in the upper panel of Fig. S3, we present the predictions of  $\text{Re}[\varepsilon_e(k_1)]$  from the approximation and those evaluated by using the Kramers-Kronig relation (S117) and  $\text{Im}[\varepsilon_e(k_1)]$  from the approximation. Similarly, in the lower panel, we compare  $\text{Im}[\varepsilon_e(k_1)]$  from the approximation with the application of Eq. (S118) to  $\text{Re}[\varepsilon_e(k_1)]$  from the approximation. Computing the Kramers-Kronig relations, we carry out numerical integrals with an upper limit of  $q = 400$ . In both panels, the strong-contrast approximation and its transformations via the Kramers-Kronig relations show excellent agreement, which numerically confirms our proof. Note that in the upper panel, there are small deviations between the approximation and its transform via the Kramers-Kronig relations. Such differences result from the fact that a finite upper limit is used to compute Eq. (S117), and the numerator  $q \text{Im}[\varepsilon_e(q)]$  in the integrand of Eq. (S117) goes to zero slowly as  $q$  increases.

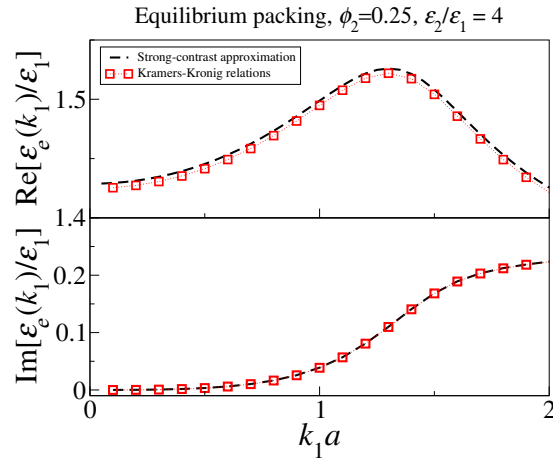

FIG. S3. Numerical verification of the Kramers-Kronig relations for the (unscaled) strong-contrast approximation. We consider 3D equilibrium packing of packing fraction  $\phi_2 = 0.25$  and contrast ratio  $\varepsilon_2/\varepsilon_1 = 4$ . In the upper panel, we compare the real part  $\text{Re}[\varepsilon_e(k_1)]$  of the approximation to that evaluated from the Kramers-Kronig relation (S117) and the imaginary part of the strong-contrast approximation. In the lower panel, we compare the imaginary part  $\text{Im}[\varepsilon_e(k_1)]$  of the approximation to that evaluated from (S118) and the real part of the approximation. The predictions from the approximation and its transform via Kramers-Kronig relations show excellent agreement.

## VI. COMPARISONS OF THE STRONG-CONTRAST APPROXIMATION WITH THE POPULAR EFFECTIVE-MEDIUM APPROXIMATIONS

We compare the asymptotic behaviors of the “unmodified” strong-contrast approximation to those of the popular effective-medium approximations [i.e., the Maxwell-Garnett approximation (MGA) and the quasicrystalline approximation (QCA)] that are employed in Sec. III in the main text. For simplicity, we consider statistically isotropic sphere packings of sphere radius  $a$  in three dimensions, where the matrix (reference) phase is taken as phase 1. We analytically demonstrate that in the quasistatic (small- $k_1$ ) and dilute regimes, MGA and QCA become consistent with the strong-contrast approximation.

We first consider the expressions in the quasistatic regime for these three approximations. For the strong-contrast approximation, by taking the Taylor expansions of Eqs. (S91) and (S92) in terms of  $Q$ , we obtain

$$F(Q) = -\frac{1}{\sqrt{2\pi}} \left[ 2 \int_0^\infty r \chi_V(r) dr Q^2 + \frac{i}{2\pi} \tilde{\chi}_V(0) Q^3 \right] + \mathcal{O}(Q^4). \quad (\text{S119})$$

Substituting Eq. (S119) and the identity  $\tilde{\chi}_V(0) = (4\pi a^3/3)\phi_2 S(0)$  into the strong-contrast approximation gives the following small- $k_1$  asymptotic expression:

$$\varepsilon_e(k_1)/\varepsilon_1 = 1 + \frac{3\phi_2\beta_{21}}{1-\phi_2\beta_{21}} + 3\phi_2 \left( \frac{\beta_{21}}{1-\phi_2\beta_{21}} \right)^2 \left[ \frac{2}{\phi_2} \int_0^\infty r \chi_V(r) dr k_1^2 + i \frac{2}{3} S(0) (k_1 a)^3 \right] + \mathcal{O}(k_1^4), \quad (\text{S120})$$

where  $\beta_{21}$  is given in Eq. (S2). The analogous expressions for the MGA and QCA are

$$\varepsilon_e(k_1)/\varepsilon_1 = 1 + \frac{3\phi_2\beta_{21}}{1-\phi_2\beta_{21}} + \frac{3\phi_2\beta_{21}^2}{1-\phi_2\beta_{21}} \left[ -\frac{1-4\beta_{21}}{5} (k_1 a)^2 + \frac{2}{3} i (k_1 a)^3 \right] + \mathcal{O}(k_1^4), \quad (\text{S121})$$

and

$$\varepsilon_e(k_1)/\varepsilon_1 = 1 + \frac{3\phi_2\beta_{21}}{1-\phi_2\beta_{21}} + 3\phi_2 \left( \frac{\beta_{21}}{1-\phi_2\beta_{21}} \right)^2 S(0) \times i \frac{2}{3} (k_1 a)^3, \quad (\text{S122})$$

respectively. We note that the static limits of these three approximations are identical to the Hashin-Shtrikman estimate

$$\varepsilon_{\text{HS}} \equiv \varepsilon_1 \left[ 1 + \frac{3\phi_2\beta_{21}}{1-\phi_2\beta_{21}} \right]. \quad (\text{S123})$$

Furthermore, the leading-order terms of  $\text{Im}[\varepsilon_e(k_1)]$  given in the strong-contrast approximation (S120) and the QCA (S122) are identical.

We now further assume the dilute limits (i.e.,  $\phi_2 \rightarrow 0$ ) of Eqs. (S120), (S121), and (S122). For typical disordered packings in the dilute regime,  $S(Q) \approx 1$ , and thus  $\tilde{\chi}_V(Q) \approx \phi_2 \tilde{a}_2(Q; a)$ ; see Sec. IIC in the main text. Combining this approximation and Eq. (S90) gives

$$F(Q) = -\frac{3\phi_2}{128\sqrt{2\pi}(Qa)^3} \left\{ \frac{1}{3} [64(Qa)^3 + 12Qa \cos(4Qa) - 3 \sin(4Qa)] + i [32(Qa)^4 - 8(Qa)^2 - 1 + \cos(4Qa) + 4Qa \sin(4Qa)] \right\} \quad (\text{S124})$$

$$= -\frac{\phi_2}{\sqrt{2\pi}} \left[ \frac{4}{5} (Qa)^2 + i \frac{2}{3} (Qa)^3 \right] + \mathcal{O}(Q^4). \quad (\text{S125})$$

Thus, the leading-order expressions in  $\phi_2$  of the strong-contrast approximation (S120) is

$$\frac{\varepsilon_e(k_1)}{\varepsilon_1} = 1 + 3\phi_2\beta_{21} + 3\phi_2\beta_{21}^2 \left[ \frac{4}{5} (k_1 a)^2 + \frac{2}{3} i (k_1 a)^3 \right] + \mathcal{O}(\phi_2^2). \quad (\text{S126})$$

In the same regime, the analogous expressions for the MGA [Eq. (S121)] and the QCA [Eq. (S122)] are given as

$$\varepsilon_e(k_1)/\varepsilon_1 = 1 + 3\phi_2\beta_{21} + 3\phi_2\beta_{21}^2 \left[ -\frac{1-4\beta_{21}}{5} (k_1 a)^2 + \frac{2}{3} i (k_1 a)^3 \right] + \mathcal{O}(\phi_2^2), \quad (\text{S127})$$

$$\varepsilon_e(k_1)/\varepsilon_1 = 1 + 3\phi_2\beta_{21} + 3\phi_2\beta_{21}^2 \times i\frac{2}{3}(k_1a)^3 + \mathcal{O}(\phi_2^2), \quad (\text{S128})$$

respectively. Unlike Eqs. (S120)-(S122) in the quasistatic regime, the leading-order terms of  $\text{Im}[\varepsilon_e(k_1)]$  given in Eqs. (S126), (S127), and (S128) are identical. This difference arises from the fact that the MGA neglects the spatial correlations of particles and is consequently operative in the dilute regime.

## VII. SIMULATION DETAILS

Here we provide additional details about simulation procedures and values of the simulation parameters that we used. We list parameters employed to generate sphere packings for computing the spectral density and the attenuation functions in Sec. VII A. We list the parameters employed in the finite-difference time-domain (FDTD) simulations in Sec. VII B. In Sec. VII C, we describe the numerical homogenization estimates obtained by FDTD simulations. In Sec. VII D, we confirm the validity of the aforementioned scheme.

### A. Parameters for Numerically Generated Packings

Here, we list the parameters employed in generating sphere packings numerically. These packings have been used to compute the spectral density (Table S1) and carry out FDTD simulations (Table S2).

We numerically generate packings for disordered stealthy hyperuniform/nonhyperuniform packings for  $d = 2, 3$ , equilibrium packings for  $d = 2$ , and hyperuniform polydisperse packings for  $d = 2, 3$  to compute the spectral density  $\tilde{\chi}_V(Q)$ ; see Sec. V in the main text. For each model, we generate  $N_c$  different packings of particle radius  $a$ ,  $N$  particles, and number density  $\rho$  in a periodic fundamental cell. Here, we list these parameters as well as some other relevant parameters.

Stealthy hyperuniform/nonhyperuniform packings are generated via the collective-coordinate optimization technique. For these models, parameters  $Q_L$  and  $Q_U$  define the stealthy regions, and  $\sigma$  represents the diameter of the repulsion region of each particle. For stealthy packings (or point patterns), it is useful to define the  $\chi$  parameter, which is the ratio of constrained degrees of freedom to total number of degrees of freedom [10, 11], i.e.,

$$\chi \equiv \frac{\mathcal{M}}{d(N-1)}. \quad (\text{S129})$$

For  $0 < \chi < 1/2$ , they are highly degenerate and disordered, whereas for  $1/2 < \chi < 1$  they crystallize [11].

Equilibrium packings for  $d = 2$  are generated via Monte Carlo simulations. We obtain hyperuniform polydisperse packings by applying the tessellation-based procedure [12, 13] to equilibrium packings of  $\phi_2 = 0.45$ . Simulation parameters employed to generate these systems are listed in Table S1.

TABLE S1. Parameters of disk/sphere packings used to compute  $\tilde{\chi}_V(Q)$ . We generate realizations of disordered stealthy hyperuniform/nonhyperuniform packings ( $d = 2, 3$ ), equilibrium packings ( $d = 2$ ), and hyperuniform polydisperse packings ( $d = 2, 3$ ). For each model,  $N_c$  is the number of distinct packings,  $N$  particle number,  $a$  is particle radius,  $\rho$  is the number density, and  $\phi_2$  is the packing fraction. For hyperuniform polydisperse packings,  $a$  stands for the mean particle radius, i.e.,  $a \equiv [\phi_2/v_1(1)]^{1/d}$ . Quantities  $Q_L$ ,  $Q_U$ , and  $\sigma$  are parameters used in the collective-coordinate optimization method; see Sec. V in the main text. The  $\chi$  parameter is defined in Eq. (S129).

| Systems \ Parameters                                      | $N$  | $\rho$ | $N_c$ | $(Q_L a, Q_U a)$ | $\sigma$ | $a$    | $\chi$ |
|-----------------------------------------------------------|------|--------|-------|------------------|----------|--------|--------|
| 2D Stealthy hyperuniform packings ( $\phi_2 = 0.25$ )     | 1000 | 1      | 300   | (0, 1.3)         | 0.57     | 0.2801 | 0.4214 |
| 3D Stealthy hyperuniform packings ( $\phi_2 = 0.25$ )     | 1000 | 1      | 300   | (0, 1.5)         | 0.8      | 0.3908 | 0.1582 |
| 3D Stealthy hyperuniform packings ( $\phi_2 = 0.4$ )      | 1000 | 1      | 300   | (0, 1.5)         | 0.92     | 0.4571 | 0.1031 |
| 2D Stealthy nonhyperuniform packings ( $\phi_2 = 0.25$ )  | 1000 | 1      | 300   | (0.9, 1.3)       | 0.57     | 0.2801 | 0.2202 |
| 3D Stealthy nonhyperuniform packings ( $\phi_2 = 0.25$ )  | 1000 | 1      | 300   | (1.0, 1.3)       | 0.8      | 0.3908 | 0.1154 |
| 2D Equilibrium packings ( $\phi_2 = 0.25$ )               | 1000 | 1      | 300   | -                | -        | 0.2801 | -      |
| 2D Hyperuniform polydisperse packings ( $\phi_2 = 0.25$ ) | 1000 | 1      | 300   | -                | -        | 0.2801 | -      |
| 3D Hyperuniform polydisperse packings ( $\phi_2 = 0.25$ ) | 1000 | 1      | 300   | -                | -        | 0.3908 | -      |

TABLE S2. Parameters of disk/sphere packings that are numerically generated for FDTD simulations. We consider simple square/cubic lattice packings, disordered stealthy hyperuniform packings, and equilibrium packings in two and three dimensions. For each model,  $N_c$  distinct packings are considered, each of which contains  $N$  particles of radius  $a$  and has number density  $\rho$ . All packings have the identical packing fraction  $\phi_2 = 0.25$ . Quantities  $Q_U$  and  $\sigma$  are the parameters for the collective-coordinate optimization method; see Sec. V in the main text.

| Systems \ Parameters              | $N$  | $\rho$ | $N_c$ | $Q_U a$ | $\sigma$ | $a$    |
|-----------------------------------|------|--------|-------|---------|----------|--------|
| Square lattice packings           | 25   | 1      | 1     | -       | -        | 0.2801 |
| Cubic lattice packings            | 25   | 1      | 1     | -       | -        | 0.3908 |
| 2D Stealthy hyperuniform packings | 100  | 1      | 20    | 1.3     | 0.57     | 0.2801 |
| 3D Stealthy hyperuniform packings | 1000 | 1      | 10    | 1.5     | 0.8      | 0.3908 |
| 2D Equilibrium packings           | 100  | 1      | 20    | -       | -        | 0.2801 |
| 3D Equilibrium packings           | 1000 | 1      | 10    | -       | -        | 0.3908 |

Table S2 lists the parameters to generate packings employed in FDTD simulations. We consider periodic packings (square and simple-cubic lattice packings) and some disordered packings (equilibrium packing and stealthy hyperuniform packings) of packing fraction  $\phi_2 = 0.25$  in two and three dimensions. For each model, we generate  $N_c$  distinct packings of unit number density ( $\rho = 1$ ) and  $N$  particles.

### B. Parameters for FDTD simulations

TABLE S3. Parameters employed in FDTD simulations via MEEP (see Sec. VII in the main text). Here  $\Delta x$  is the grid resolution,  $\rho$  is the number density of each configuration, and  $\min[k_1]$  and  $\max[k_1]$  refer to the minimal and the maximal wavenumbers of the Gaussian pulses in the matrix phase, respectively. We use different parameters for periodic and disordered models.

| Parameters            | 2D Periodic   | 3D Periodic   | 2D Disordered | 3D Disordered |
|-----------------------|---------------|---------------|---------------|---------------|
| $L$                   | 1             | 1             | 10            | 10            |
| $\Delta x \rho^{1/d}$ | 1/60          | 1/60          | 1/60          | 1/40          |
| $L_{\text{pml}}$      | 5             | 5             | 2.5           | 10            |
| $L_{\text{padd}}$     | 1             | 1             | 5             | 5             |
| $L_{\text{boundary}}$ | $\rho^{-1/2}$ | $\rho^{-1/3}$ | $\rho^{-1/2}$ | $\rho^{-1/3}$ |
| $\min[k_1]a$          | $0.1a/L$      | $0.1a/L$      | 0.1           | 0.1           |
| $\max[k_1]a$          | $4.0a/L$      | $4.0a/L$      | 1.1           | 1.1           |

We list the parameters employed to carry out FDTD simulations. Using the numerically generated packings (see Table S2), we perform FDTD simulations via MEEP, an open-source software package [14]. The simulation setup is depicted in Sec. VII in the main text. For simplicity, we take  $\varepsilon_1 = 1$  throughout the simulation. Table S3 lists the parameters employed the simulation via MEEP.

### C. Computation of $\varepsilon_e$ from FDTD simulations

Here, we provide a detailed description of numerical homogenization estimates obtained from FDTD simulations. To understand this step, we employ the concept of *macroscopic fields*, which has been used to explain the atomic origin of dielectric constants of materials [4].

At macroscopic length scales, local electric field  $\mathbf{E}^{(\text{local})}(\mathbf{x}; \omega)$  at a frequency  $\omega$  in a composite [i.e., a solution of Eq. (S24)] can be coarse-grained to macroscopic electric field  $\mathbf{E}^{(\text{macro})}(\mathbf{x}; \omega)$  defined as

$$\mathbf{E}^{(\text{macro})}(\mathbf{x}; \omega) \equiv f(\mathbf{x}) \otimes \mathbf{E}^{(\text{local})}(\mathbf{x}; \omega) = \int f(\mathbf{x} - \mathbf{x}') \mathbf{E}^{(\text{local})}(\mathbf{x}'; \omega) d\mathbf{x}', \quad (\text{S130})$$

where  $\otimes$  denotes the convolution operator,  $f(\mathbf{x})$  is a certain weighting function satisfying  $\int f(\mathbf{x}) d\mathbf{x} = 1$ , such as Gaussian distribution. Note that the support of  $f(\mathbf{x})$  is larger than the inhomogeneity length scales  $\ell$  of a composite.

Analogously, we can also define the macroscopic electric displacement field  $\mathbf{D}^{(\text{macro})}(\mathbf{x}; \omega)$  in terms of its local counterpart  $\mathbf{D}^{(\text{local})}(\mathbf{x}; \omega)$ . When the effective-medium description is valid and the medium is macroscopically isotropic (i.e.,  $\boldsymbol{\varepsilon}_e = \varepsilon_e \mathbf{I}$ ),  $\mathbf{E}^{(\text{macro})}(\mathbf{x}; \omega)$  should meet the effective wave equation

$$\nabla \times \nabla \times \mathbf{E}^{(\text{macro})}(\mathbf{x}; \omega) - k_e^2 \mathbf{E}^{(\text{macro})}(\mathbf{x}; \omega) = 0, \quad (\text{S131})$$

where  $k_e$  is the effective wavenumber in a composite at a frequency  $\omega$ . The corresponding effective dielectric constant  $\varepsilon_e$  is

$$\varepsilon_e = (k_e c / \omega)^2, \quad (\text{S132})$$

where  $c$  is the speed of light in vacuum.

From Eq. (S131), we can write the  $y$  components of macroscopic electric and electric displacement fields propagating through a composite in the  $+x$  direction as

$$\begin{aligned} E_y^{(\text{macro})}(\mathbf{x}, \omega) &\sim E_y^{(\text{macro})}(\omega) e^{ik_e \hat{\mathbf{x}} \cdot \mathbf{x}}, \\ D_y^{(\text{macro})}(\mathbf{x}, \omega) &\sim D_y^{(\text{macro})}(\omega) e^{ik_e \hat{\mathbf{x}} \cdot \mathbf{x}}, \end{aligned}$$

respectively. (While in a rigorous sense, one also needs a counter-propagating plane wave  $e^{-ik_e \hat{\mathbf{x}} \cdot \mathbf{x}}$  to describe the macroscopic fields  $E_y^{(\text{macro})}(\mathbf{x}, \omega)$  and  $D_y^{(\text{macro})}(\mathbf{x}, \omega)$ , we omit indicating it because the Fourier transforms  $\tilde{E}_y^{(\text{macro})}(k_e, \omega)$  and  $\tilde{D}_y^{(\text{macro})}(k_e, \omega)$  used in the final result (S134) are independent of the contribution from  $e^{-ik_e \hat{\mathbf{x}} \cdot \mathbf{x}}$ .) The convolution theorem yields that the spatial Fourier transforms of these macroscopic fields [e.g., Eq. (S130)] are given as

$$\begin{aligned} \tilde{E}_y^{(\text{macro})}(k_e, \omega) &\sim E_y^{(\text{macro})}(\omega) = \tilde{f}(k_e) \tilde{E}_y^{(\text{local})}(k_e, \omega), \\ \tilde{D}_y^{(\text{macro})}(k_e, \omega) &\sim D_y^{(\text{macro})}(\omega) = \tilde{f}(k_e) \tilde{D}_y^{(\text{local})}(k_e, \omega), \end{aligned}$$

where the Fourier transform is defined in the region  $V$  of a composite whose volume is  $|V|$ :

$$\tilde{h}(q) \equiv \frac{1}{|V|} \int_V h(\mathbf{x}) e^{-iq \hat{\mathbf{x}} \cdot \mathbf{x}} d\mathbf{x}. \quad (\text{S133})$$

Thus, the effective dielectric constant can be written as

$$\varepsilon_e = \frac{D_y^{(\text{macro})}(\omega)}{E_y^{(\text{macro})}(\omega)} = \frac{\tilde{D}_y^{(\text{macro})}(k_e, \omega)}{\tilde{E}_y^{(\text{macro})}(k_e, \omega)} = \frac{\tilde{D}_y^{(\text{local})}(k_e, \omega)}{\tilde{E}_y^{(\text{local})}(k_e, \omega)}, \quad (\text{S134})$$

regardless of a choice of the weighting function  $f(x)$ .

Note that the effective dielectric constants given in Eqs. (S132) and (S134) are identical provided the exact value of  $k_e$ . Since it is not easy to compute  $k_e$  in practice, however, we numerically solve the following equation of a complex wavenumber  $q$ :

$$\left| \frac{\tilde{D}_y^{(\text{local})}(q, \omega)}{\tilde{E}_y^{(\text{local})}(q, \omega)} - \left( \frac{qc}{\omega} \right)^2 \right|^2 = 0, \quad (\text{S135})$$

where the first and second terms come from Eqs. (S134) and (S132), respectively. The estimated effective dielectric constant  $\varepsilon_e$  is obtained from  $(q'c/\omega)^2$ , where  $q'$  is a solution of Eq. (S135). Clearly, the final result for  $\varepsilon_e$  obtained from Eq. (S135) is a nonlocal quantity because the nonlocal constitutive relation (S134) is used. Importantly, one can recover the conventional volume-averaging homogenization estimates from relation (S134) by taking  $k_e = 0$ , i.e.,

$$\varepsilon_e(k_1) = \tilde{D}_y(0, \omega) / \tilde{E}_y(0, \omega).$$

However, we do not use this simple volume-averaging estimate since it is no longer valid for intermediate wavelengths ( $k_1 \rho^{-1/d} \gtrsim 0.4$ ), where  $\rho$  is the number density of the particle centers [15].

### D. Validity of Extraction Method

Here we confirm the validity of the numerical homogenization estimates from FDTD simulations (see Sec. VII in the main text and Sec. VII C) in the intermediate-wavelength regime. For this purpose, we carry out the simulations for 2D and 3D periodic packings (square and simple-cubic lattice packings) of packing fraction  $\phi_2 = 0.25$ . As noted in Sec. III A, their effective dielectric constant depend on the direction of the incident wavevector  $\mathbf{k}_1$ . For simplicity, we only consider the case where  $\mathbf{k}_1$  is aligned with one of the minimal lattice vectors, i.e.,  $\Gamma$ - $X$  direction in the first Brillouin zone. Such models enable us to validate the accuracy of our FDTD simulations because  $\varepsilon_e(\mathbf{k}_1)$  also can be accurately extracted from the lowest two photonic bands, which are calculated via MPB, an open-source software package [16]. Specifically, the band structures can be converted to  $\varepsilon_e(\omega)$  at a given frequency  $\omega$ :

$$\varepsilon_e(\omega) = \left( \frac{cK}{\omega} \right)^2, \quad (\text{S136})$$

where  $K$  is the Bloch wavenumber along the  $\Gamma$ - $X$  direction. Furthermore, such periodic packings must show two salient dielectric characteristics: see Sec. VIII in the main text.

We carry out FDTD simulations for 2D square lattice packings of  $\varepsilon_2/\varepsilon_1 = 1/4, 4$ , and 3D simple-cubic lattice packing of  $\varepsilon_2/\varepsilon_1 = 4$ ; see Sec. VII B for simulation parameters. As shown in Fig. S4, the corresponding FDTD simulation results show excellent agreement with the band-structure calculations and accurately capture both of the aforementioned features up to  $k_1 L = 4$ . This implies that our numerical homogenization estimates from FDTD simulations are valid from the infinite-wavelength limit down to intermediate wavelengths.

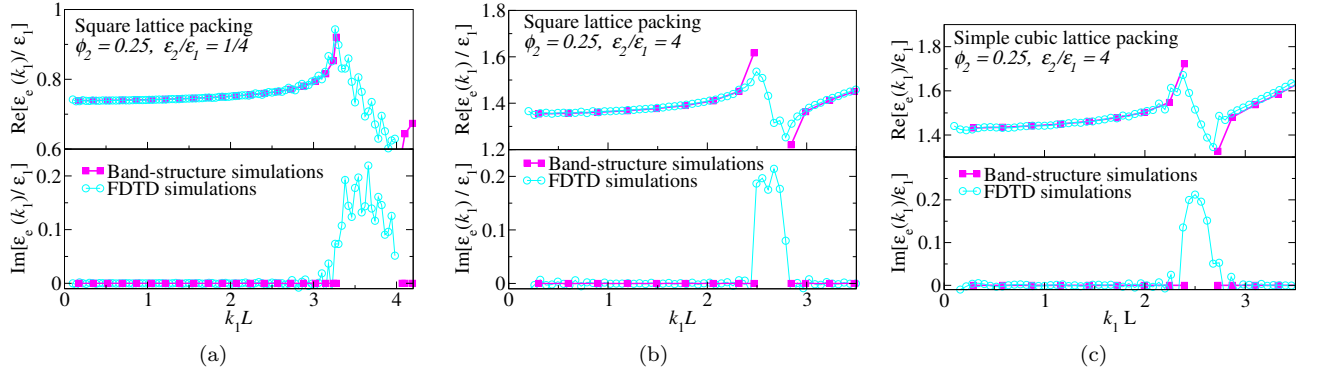

FIG. S4. Comparison of  $\varepsilon_e(k_1)$  as a function of dimensionless wavenumber  $k_1 L$  for periodic packings of  $\phi_2 = 0.25$  estimated from the band-structure (via MPB) and FDTD simulations along the  $\Gamma$ - $X$  direction. Three systems are considered: (a) square lattice packing of  $\varepsilon_2/\varepsilon_1 = 1/4$ , (b) square lattice packing of  $\varepsilon_2/\varepsilon_1 = 4$ , and (c) simple cubic lattice packing of  $\varepsilon_2/\varepsilon_1 = 4$ . Note that the band-structure calculations are omitted in the photonic bandgaps. Both types of simulations show excellent agreement, implying that our homogenization estimates from FDTD simulations are valid down to intermediate wavelengths ( $k_1 L < 4$  and  $k_1 a \lesssim 1.1$ ).

### VIII. RESULTS FOR TWO-DIMENSIONAL SYSTEMS

Here, we present some plots for two-dimensional models, which are not presented in the main text for brevity. Figure S5 shows the spectral densities and associated nonlocal attenuation functions for the four disordered models in two dimensions. All models have the same volume fraction of dispersed phase  $\phi_2 = 0.25$ .

Figure S6 compares the (both unmodified and scaled) strong-contrast approximations and the Maxwell-Garnett approximation (MGA) for the effective dielectric constant  $\varepsilon_e(\mathbf{k}_1)$  of a 2D square lattice packing to the corresponding FDTD simulation results. This packing has the packing fraction  $\phi_2 = 0.25$  and contrast ratio  $\varepsilon_2/\varepsilon_1 = 1/4$ . Similar to the results presented in the main text, the MGA shows good estimates only in the quasistatic regime. For the strong-contrast approximations, unlike the cases of  $\varepsilon_2/\varepsilon_1 > 1$ , the unmodified approximation provides better estimates for  $\text{Re}[\varepsilon_e(k_1)]$  than the scaled counterpart up to the edge of first photonic band. However, the scaled approximation correctly predicts that the frequency at which the Bragg diffraction occurs lies within the first photonic bandgap.

Figure S7 compares FDTD simulation results to the MGA and the (both unmodified and scaled) strong-contrast approximations for 2D disordered models: equilibrium packings and stealthy hyperuniform packings. Each model

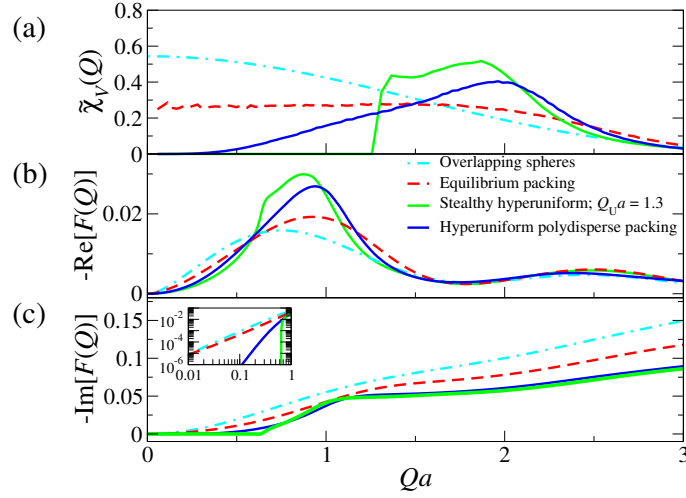

FIG. S5. Plots of (a) spectral density, and (b) the real and (c) imaginary parts of the nonlocal attenuation function as a function of dimensionless wavenumber  $Qa$  for the four models of two-dimensional disordered particulate composite media. All models have the same volume fraction of dispersed phase  $\phi_2 = 0.25$ . Here, the first three models consist of identical spheres of radius  $a$ . For class I hyperuniform packings via tessellation-based procedure,  $a$  is the mean sphere radius, i.e.,  $\phi_2 = \rho v_1(a)$ .

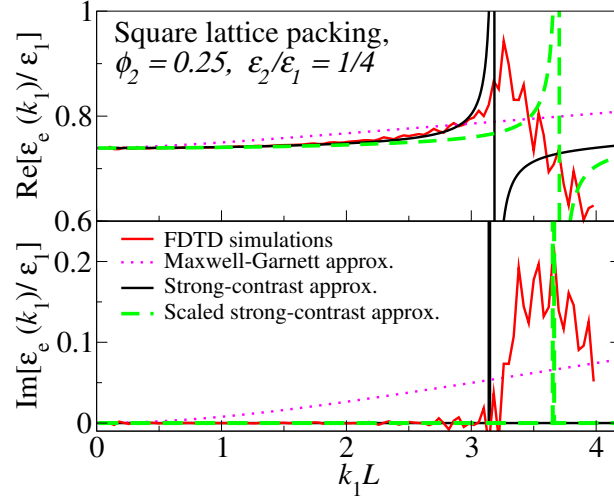

FIG. S6. Comparison of the predictions of the both scaled and unscaled strong-contrast formulas and the MGA for  $\epsilon_e(\mathbf{k}_1)$  of 2D square lattice packing to the corresponding FDTD simulation results. Packing fraction is  $\phi_2 = 0.25$ , and contrast ratio is  $\epsilon_2/\epsilon_1 = 1/4$ . Here  $k_1$  is the wavenumber in the matrix phase along the  $\Gamma$ -X direction, and  $L$  is the side length of a unit cell.

has packing fraction  $\phi_2 = 0.25$  and contrast ratio  $\epsilon_2/\epsilon_1 = 4$ . These results are qualitatively the same as the three-dimensional results discussed in the main text. Among the three approximations, the scaled strong-contrast approximation shows the best predictive power up to  $k_1 a = 0.6$ .

## IX. COMPARISON WITH MULTIPLE SCATTERING THEORY

Here we compare strong-contrast formalism to standard multiple scattering theory [6–9]. We first describe the similarities between them when they are cast in abstract linear operator form but then describe how they are generally different from one another. It is well known that for an external electric field  $\mathbf{E}_0(\mathbf{r})$  that is incident on an heterogeneous medium, the local electric field  $\mathbf{E}(\mathbf{r})$  is expressed in scattering theory as

$$\mathbf{E}(\mathbf{r}) = \mathbf{E}_0(\mathbf{r}) + \int \mathbf{G}^{(q)}(\mathbf{r}, \mathbf{r}') \cdot \mathbf{V}(\mathbf{r}') \cdot \mathbf{E}(\mathbf{r}') d\mathbf{r}', \quad (\text{S137})$$

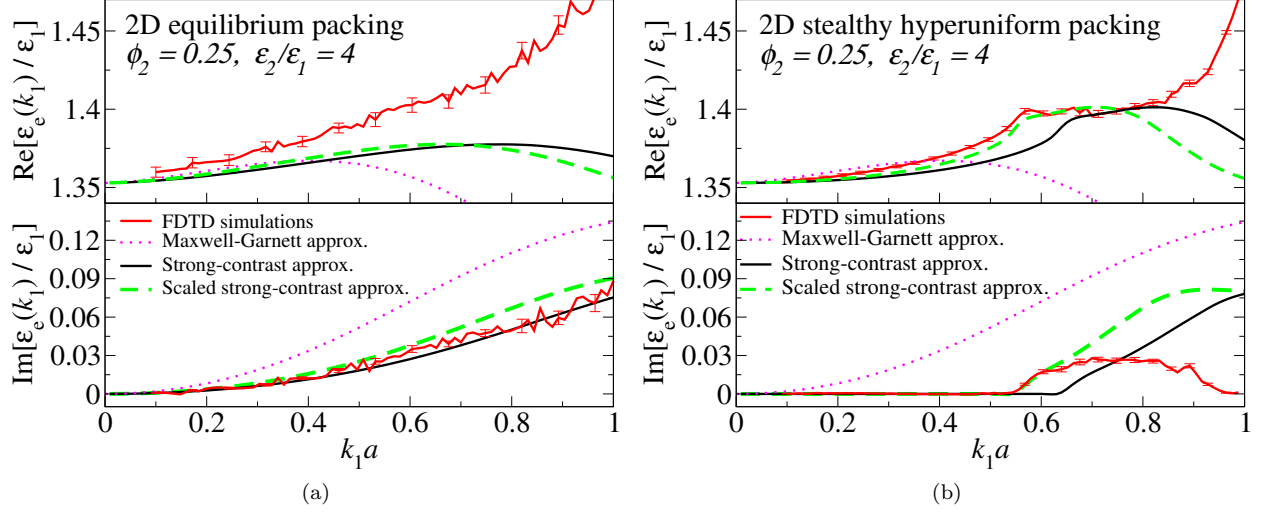

FIG. S7. Comparison of FDTD simulation results to the predictions from the strong-contrast formulas and the MGA for the effective dynamic dielectric constant  $\varepsilon_e(k_1)$  as a function of dimensionless wavenumber  $k_1 a$  of two-dimensional disordered disk packings. We consider (a) equilibrium packing and (b) stealthy hyperuniform packings [ $\tilde{\chi}_V(Q) = 0$  for  $Qa < 1.3$ ] of particle radius  $a$ , packing fraction  $\phi_2 = 0.25$ , and phase contrast ratio  $\varepsilon_2/\varepsilon_1 = 4$ . Here  $k_1$  is the wavenumber in the matrix phase, and the error bars in FDTD simulations represent the standard errors over independent configurations.

where  $\mathbf{V}(\mathbf{r}) \equiv [\varepsilon(\mathbf{r}) - \varepsilon_q]\mathbf{I}$  is the scattering potential. Note that this expression is equivalent to Eq. (S28) in the strong-contrast formalism, which uses  $\mathbf{P}(\mathbf{r}) \equiv \mathbf{V}(\mathbf{r}) \cdot \mathbf{E}(\mathbf{r})$ ; see Eq. (S25). Using the compact linear operator notation, Eq. (S137) can be expressed as

$$\mathbf{E} = \mathbf{E}_0 + \mathbf{G}\mathbf{V}\mathbf{E} \quad (\text{S138})$$

$$= \mathbf{E}_0 + \mathbf{G}\mathcal{T}\mathbf{E}_0, \quad (\text{S139})$$

where  $\mathcal{T}$  is called the *scattering operator* [6–8]. In the strong-contrast formalism, an expression corresponding to (S139) can be obtained by combining Eqs. (S28) and (S57) [see also Eqs. (23) and (37) in the main text]:

$$\mathbf{E} = \mathbf{E}_0 + \mathbf{G}\mathbf{S}\mathbf{E}_0, \quad (\text{S140})$$

where  $\mathbf{S}$  is defined in (S56) [Eq. (37) in the main text]. Comparison of Eqs. (S139) and (S140) immediately shows that the scattering operator  $\mathcal{T}$  in the multiple-scattering theory shares a common functional form with  $\mathbf{S}$  in the strong-contrast formalism, i.e.,  $\mathcal{T} = \mathbf{S}$ . However,  $\mathbf{S}$  can be regarded as a “generalized scattering operator” with superior mathematical properties compared to  $\mathcal{T}$ , as elaborated later.

Another important quantity in the multiple-scattering theory is the *self-energy operator* (also called *mass operator*)  $\Sigma(\mathbf{r}, \mathbf{r}')$ , which is defined in the Dyson equation for an ensemble average of electric field:

$$\langle \mathbf{E} \rangle = \mathbf{E}_0 + \mathbf{G}\Sigma \langle \mathbf{E} \rangle. \quad (\text{S141})$$

Comparing Eq. (S141) to an ensemble average of Eq. (S140)

$$\langle \mathbf{E} \rangle = \mathbf{E}_0 + \mathbf{G} \langle \mathbf{S} \rangle \mathbf{E}_0 = [\mathbf{I} + \mathbf{G} \langle \mathbf{S} \rangle] \mathbf{E}_0, \quad (\text{S142})$$

we immediately find a relation between  $\Sigma$  and  $\mathbf{S}$  operator:

$$\langle \mathbf{S} \rangle \mathbf{E}_0 = \Sigma \langle \mathbf{E} \rangle. \quad (\text{S143})$$

Substituting Eq. (S142) into Eq. (S143) enables us to write  $\Sigma$  in terms  $\langle \mathbf{S} \rangle$ :

$$\Sigma = \langle \mathcal{T} \rangle [\mathbf{I} + \mathbf{G} \langle \mathcal{T} \rangle]^{-1} = \langle \mathbf{S} \rangle [\mathbf{I} + \mathbf{G} \langle \mathbf{S} \rangle]^{-1}, \quad (\text{S144})$$

which also can be derived from  $\mathcal{T} = \mathbf{S}$ .

Despite these formal similarities between the multiple scattering theory and strong-contrast formalism, their results depart substantially from one another in several respects:

1. In contrast to the scattering operator  $\mathcal{T}$ , the operator  $\mathcal{S}$  acting on the applied field  $\mathbf{E}_0$  always involves an integral over the entire space such that an exclusion region (denoted by  $\int_\epsilon d\mathbf{r}$ ) is omitted [Sec. II A]; explicitly,

$$\mathcal{T}\mathbf{E}_0 \rightarrow \int \mathcal{T}(\mathbf{r}', \mathbf{r}'') \cdot \mathbf{E}_0(\mathbf{r}'') d\mathbf{r}'', \quad (\text{S145})$$

$$\mathcal{S}\mathbf{E}_0 \rightarrow \int_\epsilon \mathcal{S}(\mathbf{r}', \mathbf{r}'') \cdot \mathbf{E}_0(\mathbf{r}'') d\mathbf{r}''. \quad (\text{S146})$$

Such a difference comes from the fact that the dyadic Green's function is separated to singular and non-singular contributions (denoted by  $\mathbf{D}$  and  $\mathbf{H}$ , respectively) in the strong-contrast formalism:

$$\mathbf{G} = -\mathbf{D} + \mathbf{H}, \quad (\text{S147})$$

where  $\mathbf{D}$  depends on the exclusion-region shape; see Appendix A in the main text and Sec. II A. This general decomposition of the Green's function has huge implications for the expansion parameter that arises and the convergence properties of  $\mathcal{S}$ , as elaborated below.

2. In contrast to the multiple-scattering theory, the strong-contrast formalism has a variety of *tuning knobs* (e.g., choice of exclusion-region shape and reference phase) that enables one to obtain distinctly different expansions and approximations designed for different classes of microstructures. In this sense,  $\mathcal{S}$  can be regarded as a generalized representation of the scattering operator  $\mathcal{T}$ . Specifically,  $\mathcal{T}$  and  $\mathcal{S}$  have different representations:

$$\mathcal{T} = \mathbf{V} \sum_{n=0}^{\infty} [\mathbf{G}\mathbf{V}]^n = [\mathbf{I} - \mathbf{V}\mathbf{G}]^{-1} \mathbf{V} \quad (\text{S148})$$

$$\mathcal{S} = \mathbf{L} \sum_{n=0}^{\infty} [\mathbf{H}\mathbf{L}]^n = [\mathbf{I} - \mathbf{L}\mathbf{H}]^{-1} \mathbf{L} \quad [\text{see Eq. (S56)}], \quad (\text{S149})$$

where  $\mathbf{L} \equiv \mathbf{V}[\mathbf{I} + \mathbf{D}\mathbf{V}]^{-1} = [\mathbf{I} + \mathbf{D}\mathbf{V}]^{-1} \mathbf{V}$ ; see Eq. (S40) [(30) in the main text]. Using the definition of  $\mathbf{L}$  and Eq. (S147), it is straightforward to show that Eqs. (S148) and (S149) are identical:

$$\begin{aligned} \mathcal{S} &= \{\mathbf{I} - [\mathbf{I} + \mathbf{D}\mathbf{V}]^{-1} \mathbf{V}\mathbf{H}\}^{-1} \mathbf{L} = ([\mathbf{I} + \mathbf{D}\mathbf{V}]^{-1} \{[\mathbf{I} + \mathbf{D}\mathbf{V}] - \mathbf{V}\mathbf{H}\})^{-1} \mathbf{L} \\ &= \{[\mathbf{I} + \mathbf{D}\mathbf{V}] - \mathbf{V}\mathbf{H}\}^{-1} [\mathbf{I} + \mathbf{D}\mathbf{V}] \mathbf{L} = \{[\mathbf{I} + \mathbf{V}\mathbf{D}] - \mathbf{V}\mathbf{H}\}^{-1} [\mathbf{I} + \mathbf{D}\mathbf{V}] \mathbf{L} \\ &= \{\mathbf{I} - \mathbf{V}[-\mathbf{D} + \mathbf{H}]\}^{-1} \mathbf{V} = [\mathbf{I} - \mathbf{V}\mathbf{G}]^{-1} \mathbf{V} = \mathcal{T}. \end{aligned}$$

Since  $\mathbf{L}$  is generally a linear fractional transform of  $\mathbf{V}$ , the series (S148) and (S149) have distinctly different convergence properties, not to mention intrinsically different correlation functions. Specifically,  $\mathcal{T}$  is a series of in the simple difference  $(\varepsilon_q - \varepsilon_p)$  and thus converges slowly or cannot be applied for high contrast ratios, implying that the multiple scattering theory is essentially a “weak-contrast” expansion. By contrast, when a spherical exclusion-region is chosen,  $\mathcal{S}$  is a series of  $\beta_{pq}$ , as defined in Eq. (S2), that is bounded for any contrast ratios. For this reason, generally  $\mathcal{S}$  in the strong-contrast formalism converges substantially faster than  $\mathcal{T}$ , even for high contrast ratios. Furthermore, since  $\mathbf{L}$  depends on the choice of the exclusion-region shape, the strong-contrast formalism leads to a family of distinctly different expansions and approximations. Note that Appendix A in the main text explicitly describes other strong-contrast expansions that arise due to non-spherically shaped exclusions regions. Finally, we note that because the diagrammatic expansions of the strong-contrast formalism depend on the exclusion-exclusion shape, and it is highly nontrivial to relate them to the diagrammatic expansions in standard multiple-scattering theory.

3. Importantly, diagrammatic expansions in multiple scattering theory and strong-contrast expansions are considerably different from one another because the former is a linear fractional transform of the latter. Roughly speaking, these two theories express the self-energy  $\Sigma$  and  $[\mathbf{L}_e]^{-1}$  [see (S47) or definition (46) in the main text] as series expansions, respectively. The self-energy given in Eq. (S144) is a linear fractional transform of  $\mathbf{L}_e$ :

$$\Sigma = [\langle \mathcal{S} \rangle^{-1} + \mathbf{G}]^{-1} = [\mathbf{L}_e - \mathbf{D}]^{-1}, \quad (\text{S150})$$

where we have used  $\mathbf{L}_e = \langle \mathcal{S} \rangle^{-1} + \mathbf{H} = \langle \mathcal{S} \rangle^{-1} + \mathbf{G} + \mathbf{D}$  that is obtained from Eq. (S69). Thus, it is highly nontrivial to express the strong-contrast approximations in terms of the diagrammatic expansions in the multiple-scattering theory.

- 
- [1] M. C. Rechtsman and S. Torquato, “Effective dielectric tensor for electromagnetic wave propagation in random media,” *J. Appl. Phys.* **103**, 084901 (2008).
  - [2] A. M. Yaglom, *Correlation Theory of Stationary and Related Functions I Basic Results* (Springer-Verlag, New York, 1987).
  - [3] S. Torquato, *Random Heterogeneous Materials: Microstructure and Macroscopic Properties* (Springer-Verlag, New York, 2002).
  - [4] J. D. Jackson, *Classical Electrodynamics* (Wiley, New York, 1990).
  - [5] V. M. Agranovich and V. Ginzburg, *Crystal Optics with Spatial Dispersion, and Excitons*, 2nd ed. (Springer, Berlin, Heidelberg, 1984).
  - [6] U. Frisch, “Wave propagation in random media,” in *Probabilistic Methods in Applied Mathematics*, Vol. 1, edited by A. T. Bharucha-Reid (Academic Press, New York, 1968) 1st ed., pp. 75–198.
  - [7] P. Sheng, *Introduction to Wave Scattering, Localization and Mesoscopic Phenomena* (Academic Press, New York, 1995).
  - [8] L. Tsang, *Scattering of Electromagnetic Waves*, edited by J. A. Kong, Wiley Series in Remote Sensing (Wiley, Chichester, UK, 2001).
  - [9] A. Cazé and J. C. Schotland, “Diagrammatic and asymptotic approaches to the origins of radiative transport theory: Tutorial,” *J. Opt. Soc. Am. A* **32**, 1475 (2015).
  - [10] S. Torquato, G. Zhang, and F. H. Stillinger, “Ensemble theory for stealthy hyperuniform disordered ground states,” *Phys. Rev. X* **5**, 021020 (2015).
  - [11] G. Zhang, F. Stillinger, and S. Torquato, “Ground states of stealthy hyperuniform potentials: I. Entropically favored configurations,” *Phys. Rev. E* **92**, 022119 (2015).
  - [12] J. Kim and S. Torquato, “New tessellation-based procedure to design perfectly hyperuniform disordered dispersions for materials discovery,” *Acta Materialia* **168**, 143–151 (2019).
  - [13] J. Kim and S. Torquato, “Methodology to construct large realizations of perfectly hyperuniform disordered packings,” *Phys. Rev. E* **99**, 052141 (2019).
  - [14] A. F. Oskooi, D. Roundy, M. Ibanescu, P. Bermel, J. D. Joannopoulos, and S. G. Johnson, “Meep: A flexible free-software package for electromagnetic simulations by the FDTD method,” *Comput. Phys. Commun.* **181**, 687–702 (2010).
  - [15] V. V. Gozhenko, A. K. Amert, and K. W. Whites, “Homogenization of periodic metamaterials by field averaging over unit cell boundaries: Use and limitations,” *New J. Phys.* **15**, 043030 (2013).
  - [16] S. G. Johnson and J. D. Joannopoulos, “Block-iterative frequency-domain methods for Maxwell’s equations in a planewave basis,” *Opt. Express* **8**, 173–190 (2001).
